# Supplementary material for: Mesh Watermark Removal Attack and Mitigation: A Novel Perspective of Function Space
Source: arXiv:2311.12059 source file (2025-01-25)
Supplement: Supplementary file 1 [file supp.tex]

% 每个wm的参数

% Nv - acc, error rate
% shapenet dataset Nv distribute
% visual mesh-based

\section{Section A: Analytic Deformation} \label{sec:analytic}
Since our watermark is embedded through deforming the SDF, we provide more details of SDF deformation:
\begin{itemize}
    \item Explain details of estimating $\mathbf{y}=D^{-1}(\mathbf{x})$ by Newton's method.
    \item Conduct analytic derivation of $\nabla G_\Theta(\mathbf{x})$.
    % \item Explain why we use analytic $D(\mathbf{x})$ instead of neural $D(\mathbf{x})$, which is commonly used in prior works \cite{NFGP, deng2021deformed, liu2021editing}.
\end{itemize}

% Definition of $D(\mathbf{y})$, which deforms $\mathbf{y}$ to $\mathbf{x}=D(\mathbf{y})$:
% \begin{equation}
%     D(\mathbf{y})=
%     \begin{cases}
%         \mathbf{y}+\nabla F_\Theta(\mathbf{y})C(\mathbf{y})&b=1\\
%         \mathbf{y}-\nabla F_\Theta(\mathbf{y})C(\mathbf{y})&b=0
%     \end{cases}
%     \label{eq: D}
% \end{equation}

\textbf{Implementation details of the Newton's method.} In Alg. \ref{alg:newton}, given a deformed point $\mathbf{x}=D(\mathbf{y})$, we calculate $\mathbf{y}=D^{-1}(\mathbf{x})$ by Newton's method via a repeated iteration $\mathbf{y}_{n+1}=\mathbf{y}_{n}-\mathcal{J}^{-1}_{D}(\mathbf{y}_{n})\cdot D(\mathbf{y}_{n})$, where $\mathcal{J}_{D}(\mathbf{y})$ is a function of $\mathcal{H}_{F_\Theta}(\mathbf{y})$ and $\nabla F_\Theta(\mathbf{y})$:
\begin{equation}
    \mathcal{J}_{D}(\mathbf{y})=\mathcal{I}+\delta\mathcal{H}_{F_\Theta}(\mathbf{y})
\end{equation}
Since $\nabla F_\Theta(\mathbf{y})$ is supervised with ground truth values (\ie, vertex normals) only when $\mathbf{y}$ is a on-surface point, those $\mathcal{H}_{F_\Theta}(\mathbf{y})$ and $\nabla F_\Theta(\mathbf{y})$ may not be accurate when $\mathbf{y}$ is far from the surface. This supports the statement in our main paper that Newton's method may not find a zero point if the initialization $\mathbf{y}_0$ is far from the zero-isosurface. Hence, we initialize batched $y_{0}^{(j)}$ to find the zero point. In our experiment, we find that 100 batch size is enough to find the ground truth zero point, and we set the desired tolerance $\tau=10^{-8}$, and the maximum iteration $N_i=100$.

\begin{algorithm}
\caption{Estimating $\mathbf{y}=D^{-1}(\mathbf{x})$}\label{alg:newton}
\hspace*{\algorithmicindent} \textbf{Input} $F_\Theta$, desired tolerance $\tau$, maximum iteration $N_i$\\
\hspace*{\algorithmicindent} \textbf{Output} estimated $\mathbf{y}$
\begin{algorithmic}[1]
\State Sample batch $\{\mathbf{y}_0^{(j)}\in [-1,1]^3\}_{j\in \{0,1,...,98,99\}}$
\While{$i<N_i$ or $\forall |F_\Theta(\mathbf{y}_i^{(j)})|>\tau$}
    \ForAll{$j\in \{0,1,...,98,99\}$}
        \State $\mathbf{y}_i^{(j)} \gets \mathbf{y}_{i-1}^{(j)}-\mathcal{J}_{D}^{-1}(\mathbf{y}_{i-1}^{(j)})\cdot D(\mathbf{y}_{i-1}^{(j)})$
    \EndFor
\EndWhile
\State $\mathbf{y} \gets \argmin_{\mathbf{y}_{i}^{(j)}} |F_\Theta(\mathbf{y}_{i}^{(j)})|$
\end{algorithmic}
\end{algorithm}

\textbf{Derivation of $\nabla G_\Theta (\mathbf{x})$.} By chain rule, we have $\nabla G_\Theta(\mathbf{x})=\mathcal{J}_{D^{-1}}(\mathbf{x})\cdot \nabla F_\Theta(\mathbf{y})$, where $\mathbf{y}=D^{-1}(\mathbf{x})$. With the estimated $\mathbf{y}$ and the given $F_\Theta$, we now have the value of $\nabla F_\Theta (\mathbf{y})$ and the only unknown value $\mathcal{J}_{D^{-1}}(\mathbf{x})$. Fortunately, $\mathcal{J}_{D^{-1}}(\mathbf{x})$ can be obtained from the following derivation:
\begin{equation}
    \begin{aligned}
        \mathbf{x}=D(\mathbf{y})&=\mathbf{y}+\delta\frac{\partial F_\Theta}{\partial y}\\
        \mathcal{I}&=\frac{\partial \mathbf{y}}{\partial \mathbf{x}}+\delta\frac{\partial^2 F_\Theta}{\partial y\partial x}\\
        \mathcal{I}&=\frac{\partial \mathbf{y}}{\partial \mathbf{x}} \Bigl(\mathcal{I}+\delta\frac{\partial^2F_\Theta}{\partial y^2}\Bigr)\\
        \mathcal{J}_{D^{-1}}(\mathbf{x})&=\Bigl(\mathcal{I}+\delta\mathcal{H}_{F_\Theta}\Bigr)^{-1}
    \end{aligned}
    \label{eq:J_derive}
\end{equation}

\begin{table}[t]
    \centering
    \small
    \begin{tabular}{c|c| c}
    % \toprule[1pt]
     Function & Method & MSE Loss\\
     \hline\hline
     \multirow{2}{*}{$D(\mathbf{y})$} & neural & $0.001$\\
     & analytic & $\mathbf{0.0}$\\
     \hline
     \multirow{2}{*}{$D^{-1}(\mathbf{x})$} & neural & $0.001$\\
     & analytic & $\mathbf{3.4*10^{-9}}$\\
    \bottomrule[1pt]
    \end{tabular}
    \caption{MSE loss is evaluated between ground truth $\mathbf{x}_i$ and $D(\mathbf{y}_i)$, and between ground truth $\mathbf{y}_i$ and $D^{-1}(\mathbf{x}_i)$.}
    \label{tab:ablation}
\end{table}

\section{Section B: Analytic Deformation vs. Neural Deformation}

We get the watermarked SDF $G_\Theta(\mathbf{x})$ from the original SDF $F_\Theta$ through neural field deformation by a deformation field $D(\mathbf{y})$. Given the original point $\mathbf{y}$, we get its deformed point through $\mathbf{x}=D(\mathbf{y})$. In this case, the deformed SDF can be obtained by wrapping the coordinate space of the original SDF: $G_\Theta(\mathbf{x})=F_\Theta(D^{-1}(\mathbf{x}))$. Prior works \cite{NFGP, deng2021deformed, liu2021editing} implement the neural deformation field, \ie the deformation field $D(\mathbf{y})$ is built with an invertible neural network. Instead, we use the analytic deformation field, where our $D(\mathbf{y})$ has an explicit formula, and make it invertible through Newton's method \cite{newtonmethod}. We conduct an ablation study to show that neural $D(\mathbf{x})$ cannot satisfy the accuracy required by watermarking tasks. The neural $D(\mathbf{x})$ is built with invertible residue networks \cite{behrmann2019invertible} to make it invertible, which is the same as the one used in NFGP \cite{NFGP}. We generate ground truth $\{(\mathbf{x}_i, \mathbf{y}_i)\}$ by first sampling original points $\mathbf{y}_i$ on the surface of $F_\Theta$, and then get deformed points $\mathbf{x}_i=D(\mathbf{y}_i)$. Tab. \ref{tab:ablation} shows that the neural $D(\mathbf{y})$ cannot satisfy the accuracy requirement because the fitting error is as large as the default watermarking strength $\delta=0.001$ in our main paper.

\section{Section C: Robustness against Affine Transformation}
Affine transformation can remove the watermark easily because all points will be tagged by a wrong bit. To alleviate this issue, we align the given mesh (with vertex set $V$) with watermarked SDF $G_\Theta$ by minimizing:
\begin{equation}
    \begin{aligned}
        &(a^*,\beta^*,\theta^*,\phi^*,\mathbf{t}^*)=\\
        &\argmin_{a,\beta,\theta,\phi,\mathbf{t}}\sum_{v\in V} \lVert G_\Theta(a \mathbf{R}(\beta, \theta, \phi) v + \mathbf{t}) \rVert,\\
    \end{aligned}
    \label{eq: align_mesh_SDF}
\end{equation}
where $a$ is the scaling factor, $\mathbf{R}(\beta, \theta, \phi)$ representing the function mapping a rotation angle $\beta$ and a rotation axis $(\theta, \phi)$ to the rotation matrix, and $\mathbf{t}$ is the translation vector. 3D rotation learning is hard due to the non-continuous mapping of $\mathbf{R}$ \cite{continuity_rotaion_learning}. Gradient descent can find the global optimum only if the initialized parameter set $(\alpha,\beta,\theta,\phi,\mathbf{t})$ is close to optimum $(\alpha^*,\beta^*,\theta^*,\phi^*,\mathbf{t}^*)$. We perform a coarse-to-fine-grained parameter search. For coarse-grained search, we use grid search to find a set of initialized parameter set $(\alpha,\beta,\theta,\phi,\mathbf{t})$. We use gradient descent within each grid for a fine-grained search to find the global optimum.

\section{Section D: More Experiment Results}

The evasion rate is calculated as follows:
\begin{equation}
EVA=\frac{N_{evade}}{N_{watermarked}}
\end{equation}
where $N_{watermarked}$ denotes number of watermarked mesh, and $N_{evade}$ denotes number of post-processed meshes which evade watermark detection.

The Hausdorff distance is calculated as follows:
\begin{equation}
    \begin{aligned}
        HD(X, Y)=\max\{\sup_{x\in X} d(x, Y), \sup_{y \in Y} d(y, X)\},
    \end{aligned}
\end{equation}
where $\sup$ represents supremum operator, $X,Y$ represent two vertex set, and $d(\cdot,\cdot)$ gives the shortest distance between two inputs. When evaluating Hausdorff distance between two meshes $HD(\mathcal{M}_X, \mathcal{M}_Y)$, we are evaluating their vertex sets $HD(V_X,V_Y)$.

\noindent \textbf{Question 1.} Does \attack dominate the trade-off compared to other removal methods?

\begin{figure}[t]
    \centering
    \includegraphics[width=\linewidth]{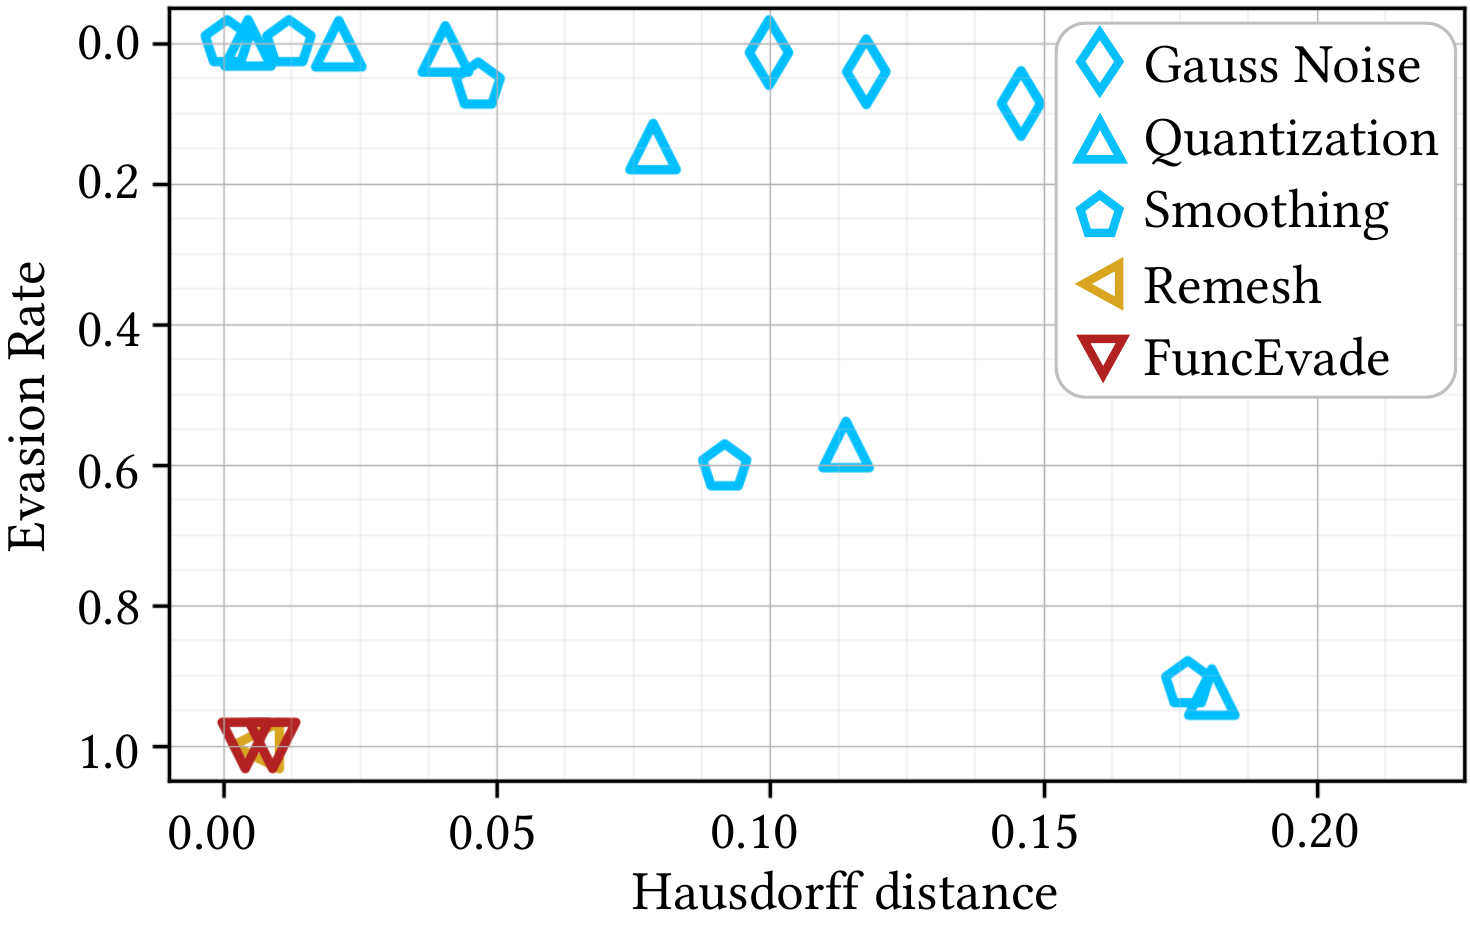}
    \caption{Trade-off between removal distortion and evasion rate. The removal attack is conducted on Deep3DMark. We varied the removal strength for all post-process methods to show that function space removal methods achieve the highest evasion rate while keeping the lowest removal distortion.}
    \label{fig:tradeoff}
\end{figure}

Fig. \ref{fig:tradeoff} shows that \attack and remeshing dominate the trade-off compared to other removal methods. A higher evasion rate results in a higher Hausdorff distance (thus lower mesh similarity). We control this trade-off by varying the removal strength of post-process methods. We control the attack strength of removal strength by varying standard deviation $\sigma\in[0.001, 0.05]$, quantization bits $N_b\in [2, 10]$, smoothing $\lambda\in[0.5, 10]$ and extraction resolution $res\in\{512, 1024\}$ from SDF. Gauss noise, quantization, and smoothing cannot achieve larger evasion rate than \attack and remeshing without limiting less Hausdorff distance than \attack and remeshing.

\noindent \textbf{Question 2.} How is the impact of different isosurfacing methods?

The watermark of \defence can be verified on the extracted meshes, which are extracted through isosurfacing. When meshes are extracted using different isosurfacing methods, the accuracy of the decoded message is expected to be high. Table \ref{tab:robustness_isosurface} shows the accuracy under different isosurfacing methods. We can observe that \defence achieves high bit accuracy under different isosurfacing methods.

\begin{table}[t]
    \centering
    \small
    \begin{tabular}{cc}
    \toprule[1pt]
     Isosurfacing & Acc\\\hline
     Marching Cubes \cite{lorensen1998MC} & 93.12\\
     Dual Contouring \cite{ju2002DC} & 87.75\\
     Neural Dual Contouring \cite{chen2022NDC} & 88.61\\
    \bottomrule[1pt]
    \end{tabular}
    \caption{Accuracy under different isosurfacing methods.}
    \label{tab:robustness_isosurface}
\end{table}

% To show our sampling strategy effectively samples the on-surface points, we provide visual results of sampled points in Fig.\ref{fig:sampling}.

% \begin{figure}[htb]
%     \centering
%     \includegraphics[width=\linewidth]{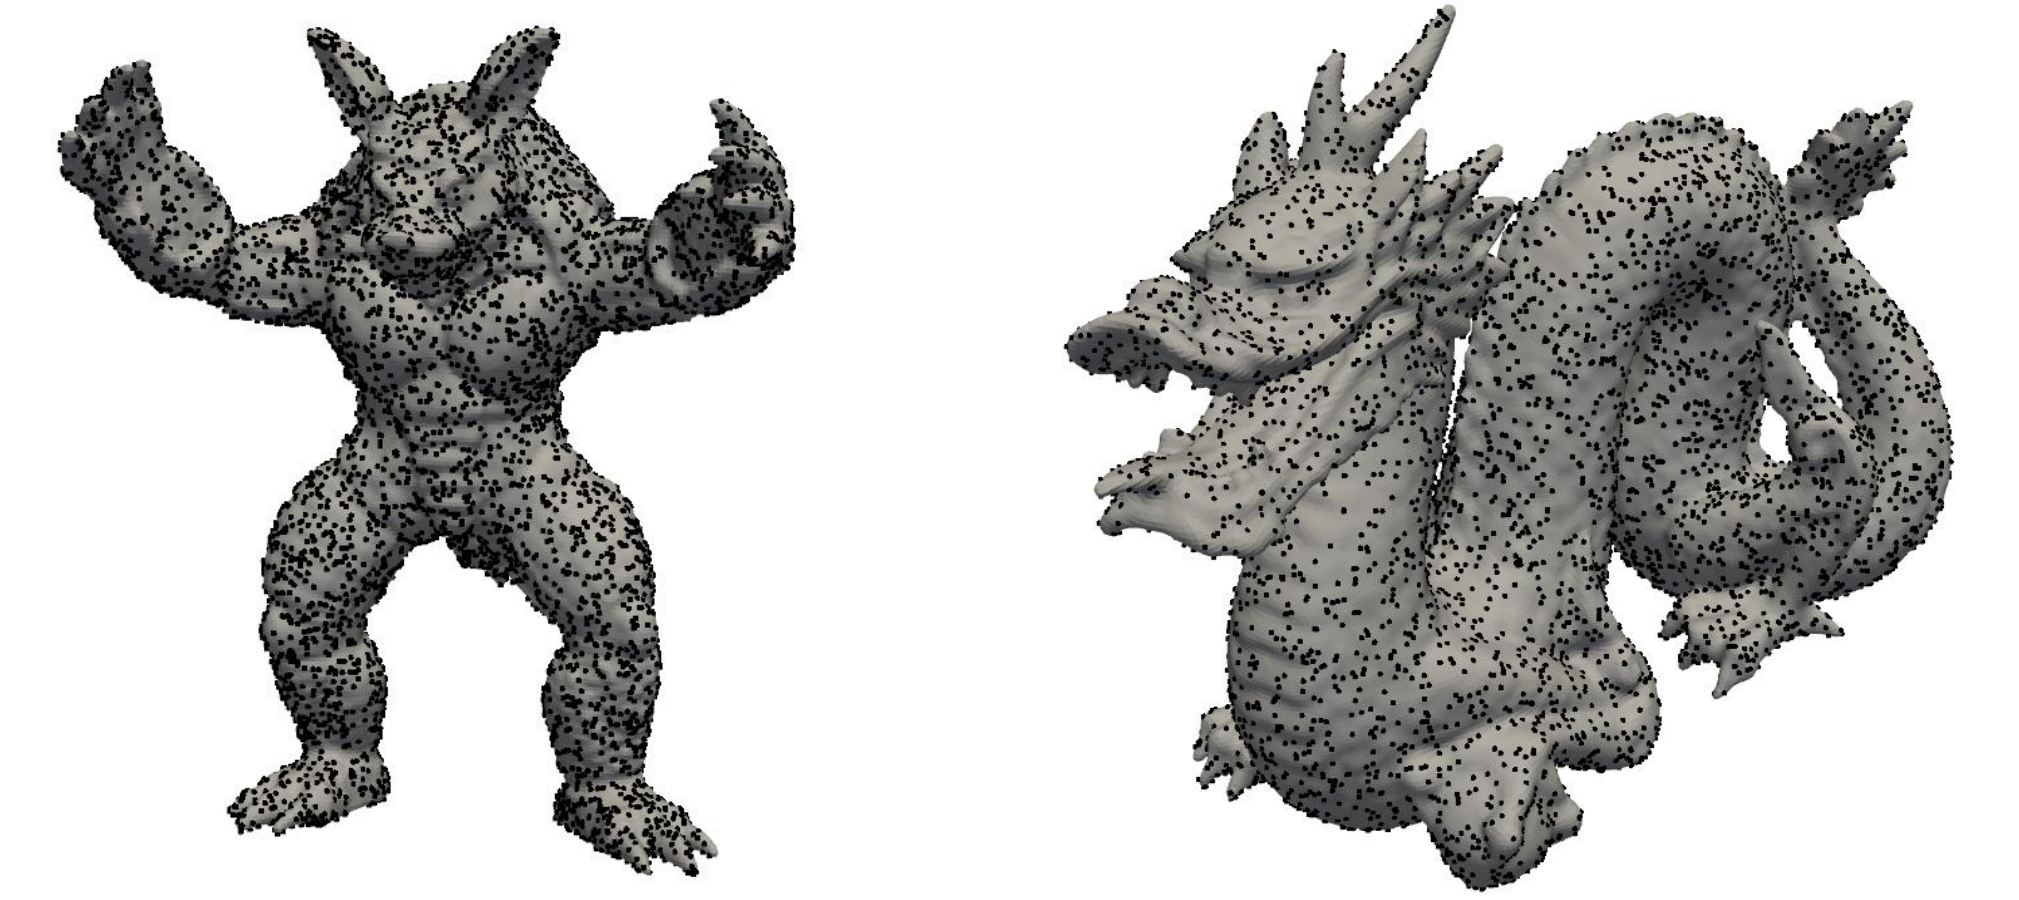}
%     \caption{SDF surface sampling.}
%     \label{fig:sampling}
% \end{figure}

% To show our fitting strategy effectively fits a high-quality signed distance function that generates high-quality meshes, we provide visual results of the mesh extracted from the fitted $F_\Theta$, the mesh extracted from watermarked $G_\Theta$ and their vertex normals $\nabla F_\Theta$ and $\nabla G_\Theta$ respectively in Fig. \ref{fig:visual_f_theta}.

% \begin{figure}[htb]
%     \centering
%     \includegraphics[width=\linewidth]{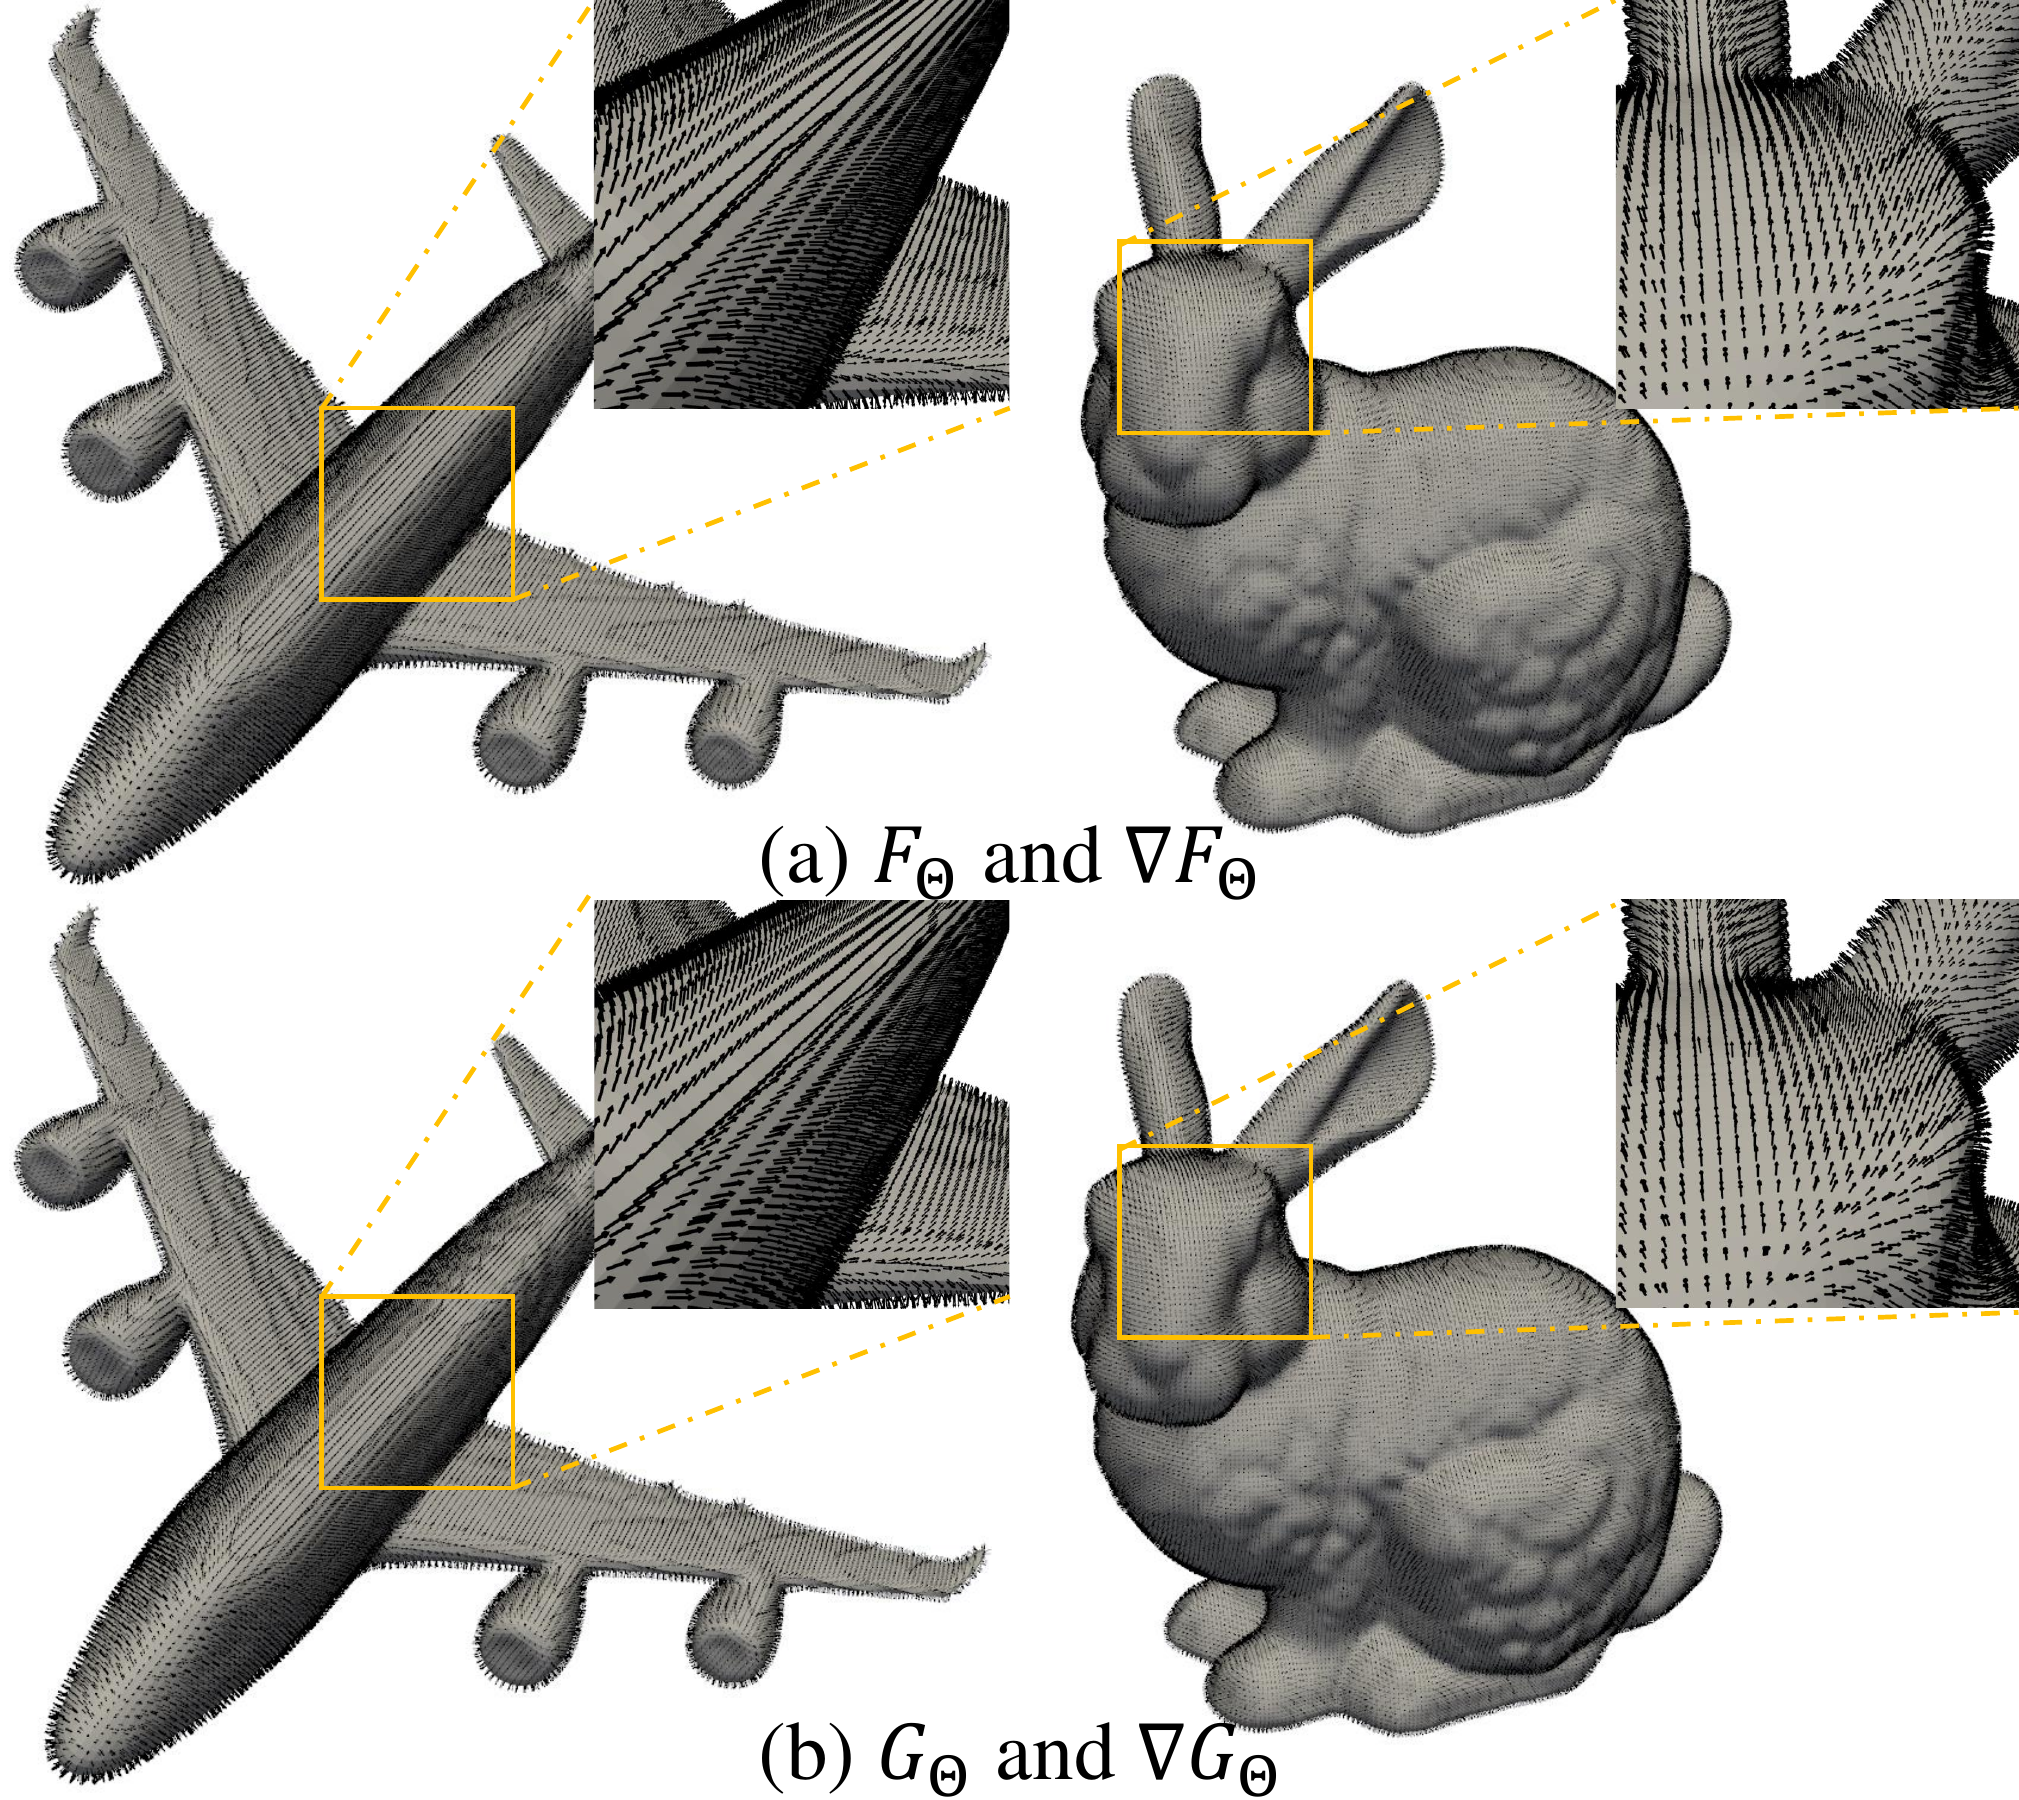}
%     \caption{Visualize $F_\Theta$, $\nabla F_\Theta$, $G_\Theta$ and $\nabla G_\Theta$.}
%     \label{fig:visual_f_theta}
% \end{figure}

\noindent \textbf{Question 3.} Show more visual results.

For watermark removal analysis, we provide more visual results of removal methods in Fig. \ref{fig:attack_more}. For function space watermarking, we provide more visual results of \defence in Fig. \ref{fig:more_visual}.

\begin{figure*}
    \centering
    \begin{subfigure}[b]{0.13\linewidth}
        \includegraphics[width=\linewidth, page=1]{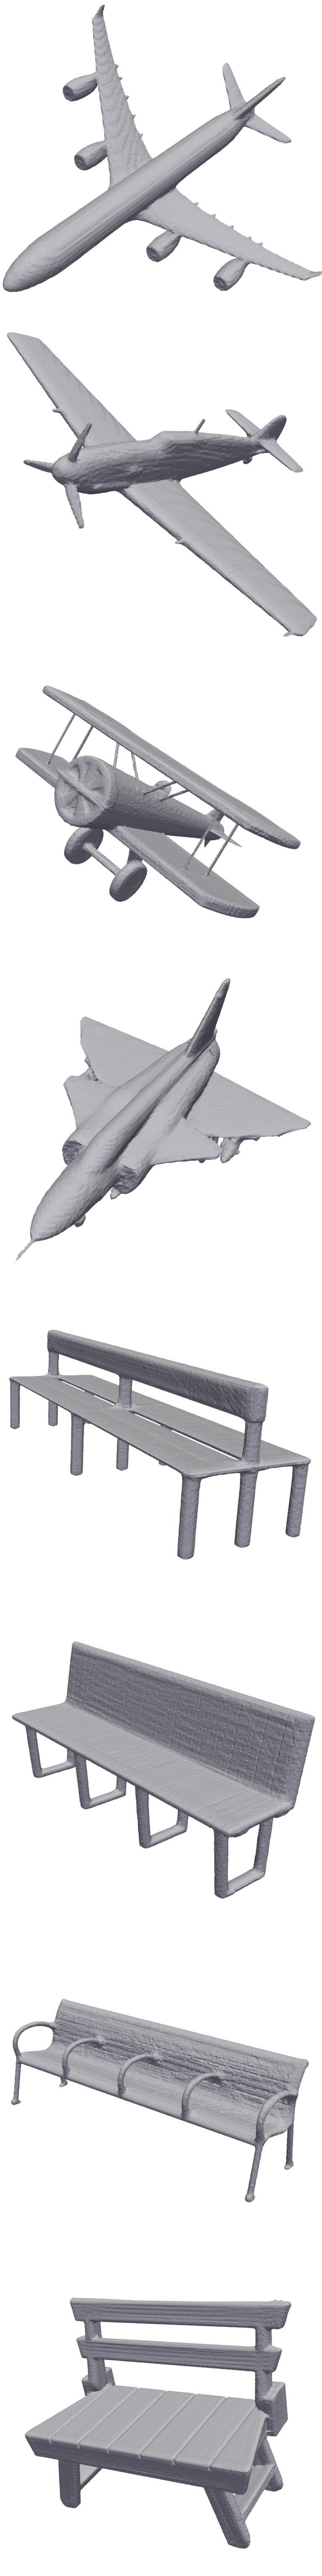}
        \caption{Original}
    \end{subfigure}
    \begin{subfigure}[b]{0.13\linewidth}
        \includegraphics[width=\linewidth, page=2]{figures/supp/attack_more.pdf}
        \caption{Watermarked}
    \end{subfigure}
    \begin{subfigure}[b]{0.13\linewidth}
        \includegraphics[width=\linewidth, page=3]{figures/supp/attack_more.pdf}
        \caption{Gauss Noise}
    \end{subfigure}
    \begin{subfigure}[b]{0.13\linewidth}
        \includegraphics[width=\linewidth, page=4]{figures/supp/attack_more.pdf}
        \caption{Quantization}
    \end{subfigure}
    \begin{subfigure}[b]{0.13\linewidth}
        \includegraphics[width=\linewidth, page=5]{figures/supp/attack_more.pdf}
        \caption{Smoothing}
    \end{subfigure}
    \begin{subfigure}[b]{0.13\linewidth}
        \includegraphics[width=\linewidth, page=6]{figures/supp/attack_more.pdf}
        \caption{Remesh}
    \end{subfigure}
    \begin{subfigure}[b]{0.13\linewidth}
        \includegraphics[width=\linewidth, page=7]{figures/supp/attack_more.pdf}
        \caption{FuncEvade}
    \end{subfigure}
    \caption{More illustration of (a) original mesh, (b) watermarked mesh, and (c-f) watermarked meshes post-processed by existing removal methods and (g) \attack to evade detection. Among all post-process methods, \attack achieves the highest evasion rate while keeping the highest post-processed mesh quality.}
    \label{fig:attack_more}
\end{figure*}

\begin{figure*}
    \centering
    \begin{subfigure}[b]{0.24\linewidth}
        \includegraphics[width=\linewidth, page=1]{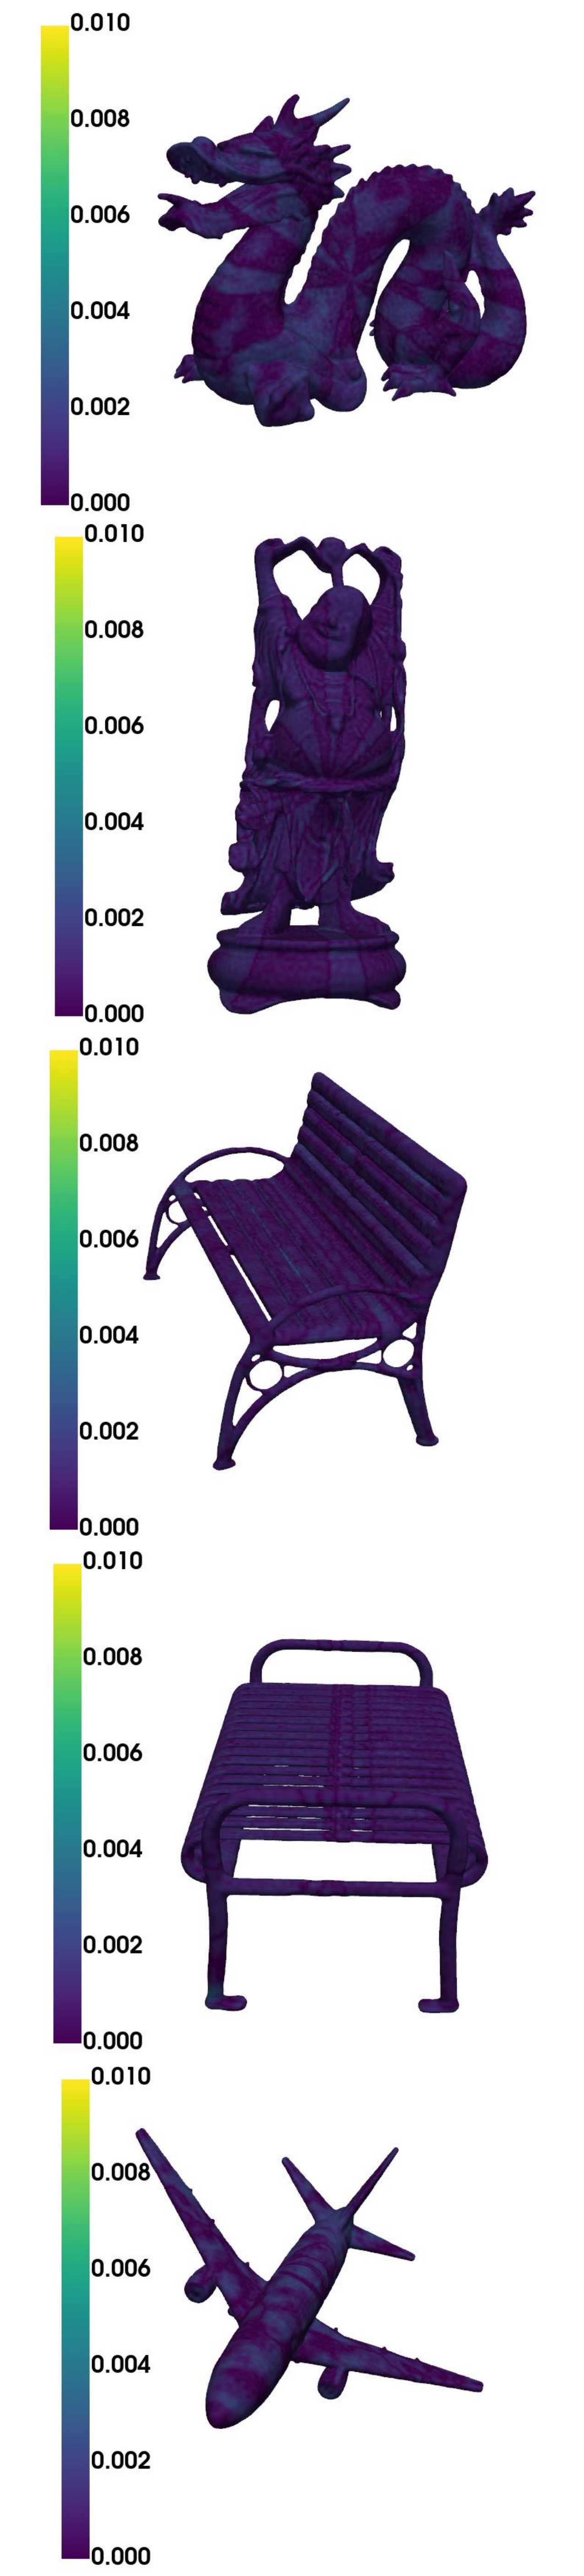}
        \caption{Shortest distance to original mesh for each vertex}
    \end{subfigure}
    \begin{subfigure}[b]{0.24\linewidth}
        \includegraphics[width=\linewidth, page=2]{figures/supp/more_visual.pdf}
        \caption{The original mesh}
    \end{subfigure}
    \begin{subfigure}[b]{0.24\linewidth}
        \includegraphics[width=\linewidth, page=3]{figures/supp/more_visual.pdf}
        \caption{Mesh extracted from $G_\Theta$}
    \end{subfigure}
    \begin{subfigure}[b]{0.24\linewidth}
        \includegraphics[width=\linewidth, page=4]{figures/supp/more_visual.pdf}
        \caption{Visualize vertex tags $b$}
    \end{subfigure}
    \caption{(a-c) Visualize geometric differences between \textit{mesh-256} from $F_\Theta$ and $G_\Theta$. (d) Vertex tags $b$ on \textit{mesh-256} from $G_\Theta$.}
    \label{fig:more_visual}
\end{figure*}
