# Supplementary material for: Mesh Watermark Removal Attack and Mitigation: A Novel Perspective of Function Space
Source: arXiv:2311.12059 source file (2025-01-25)

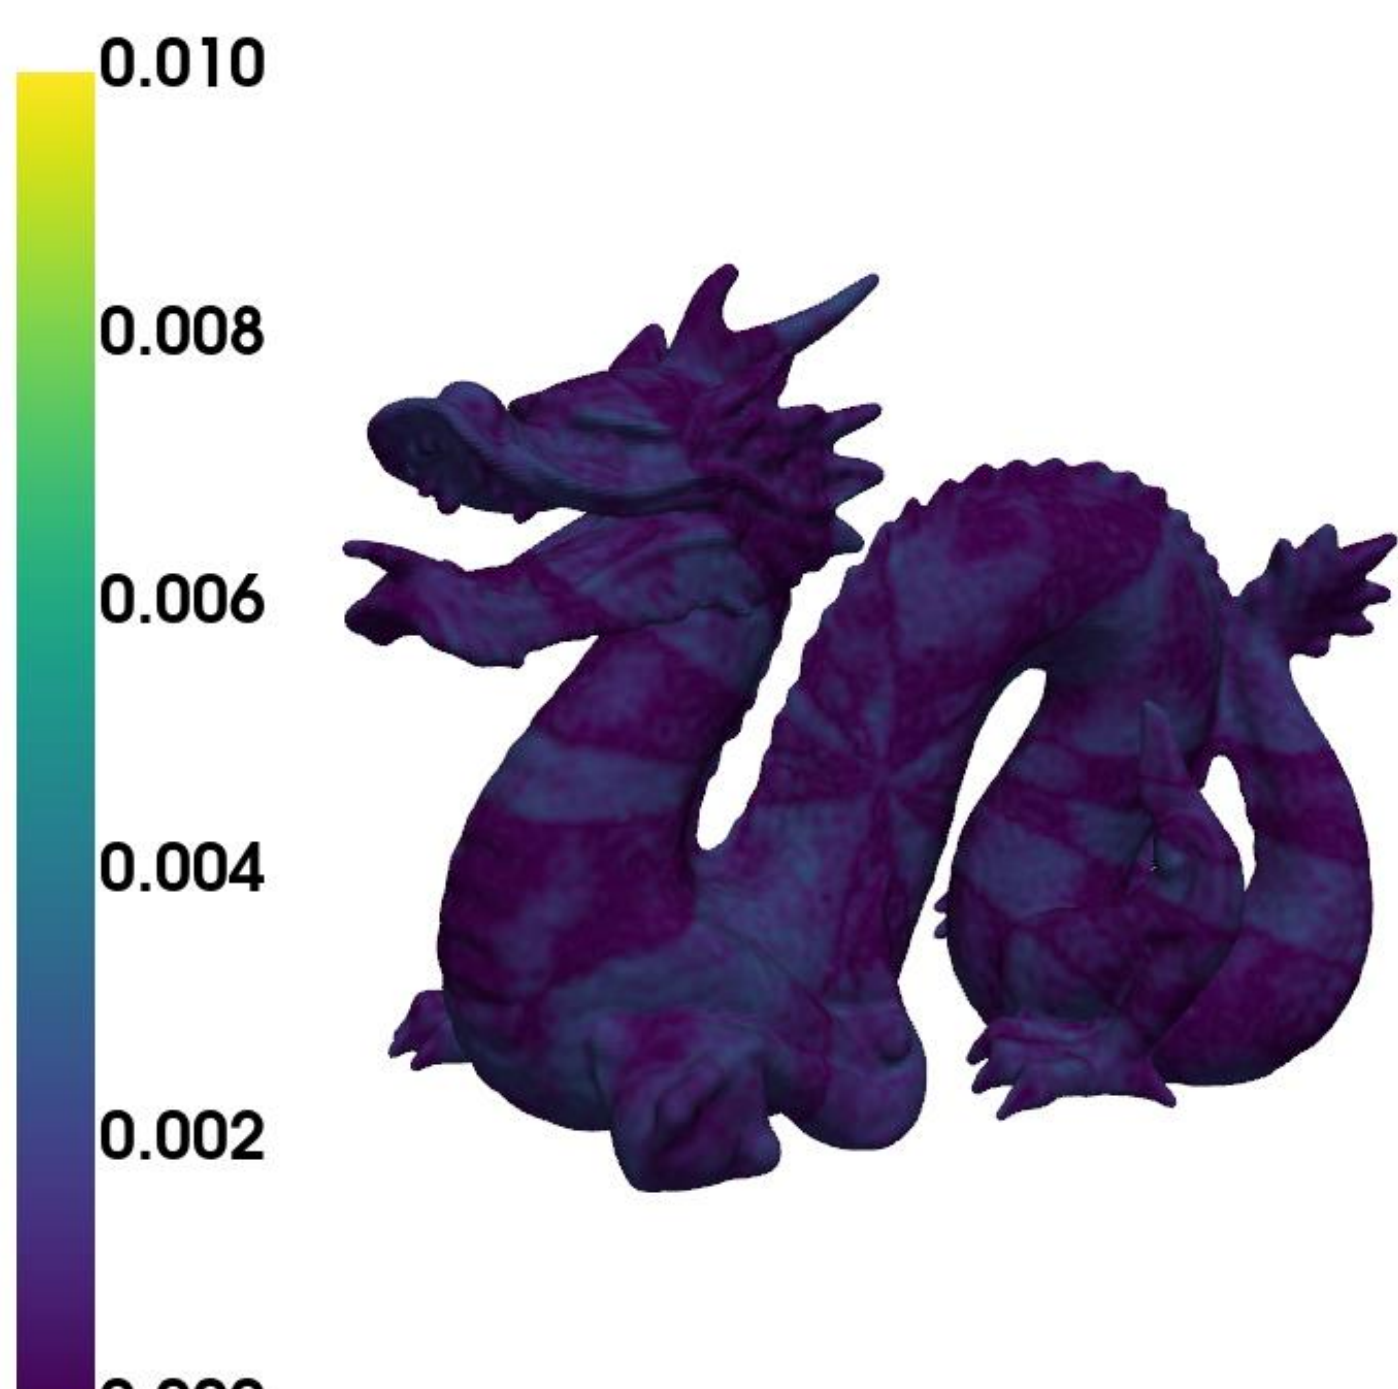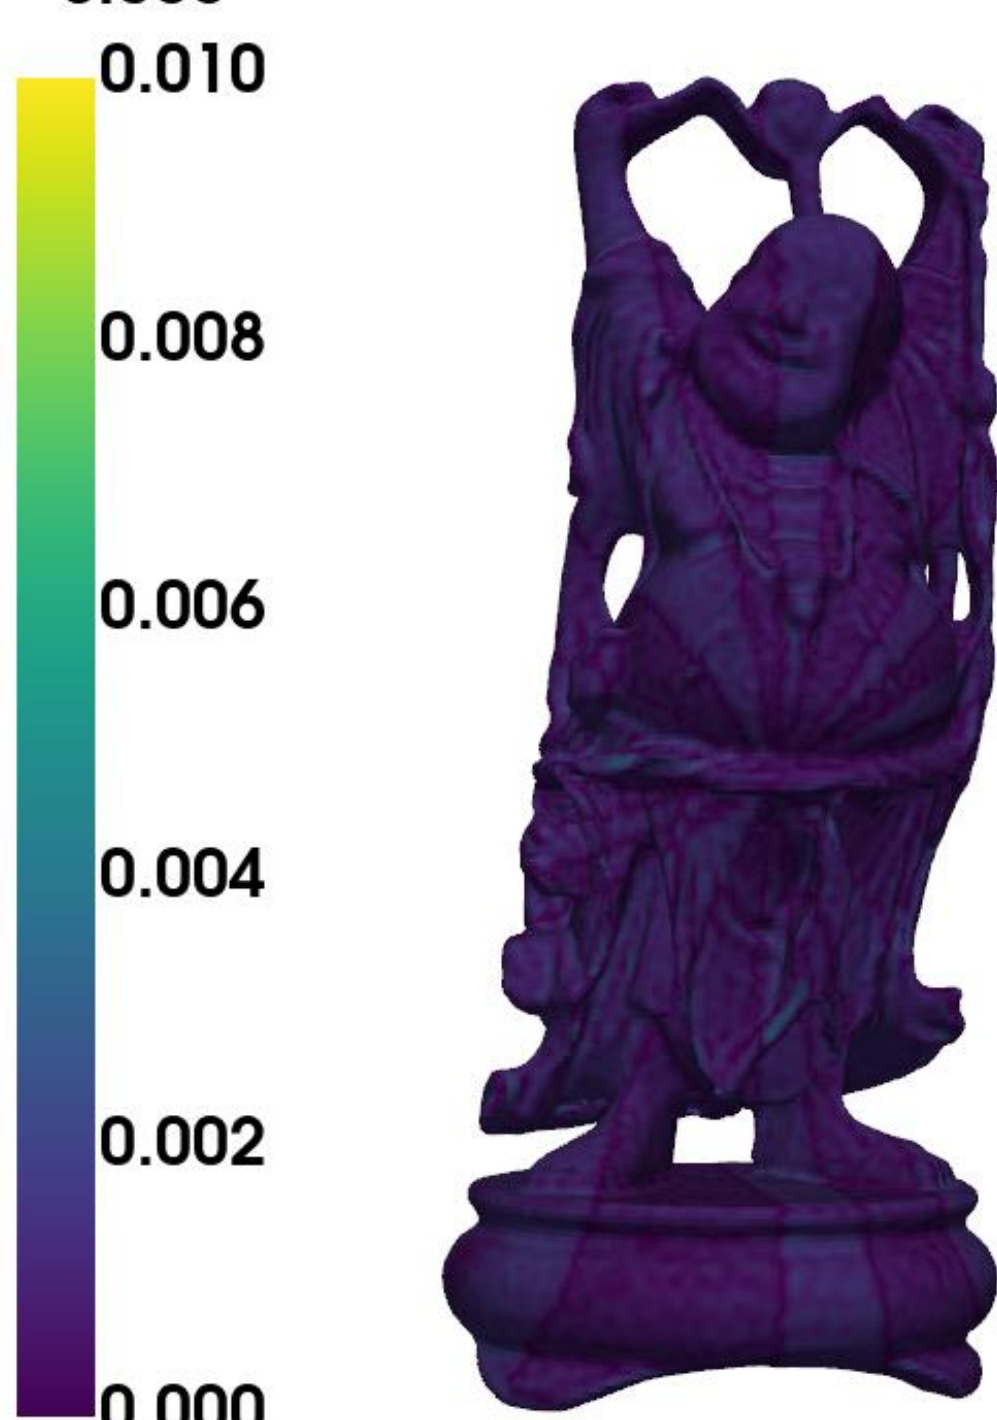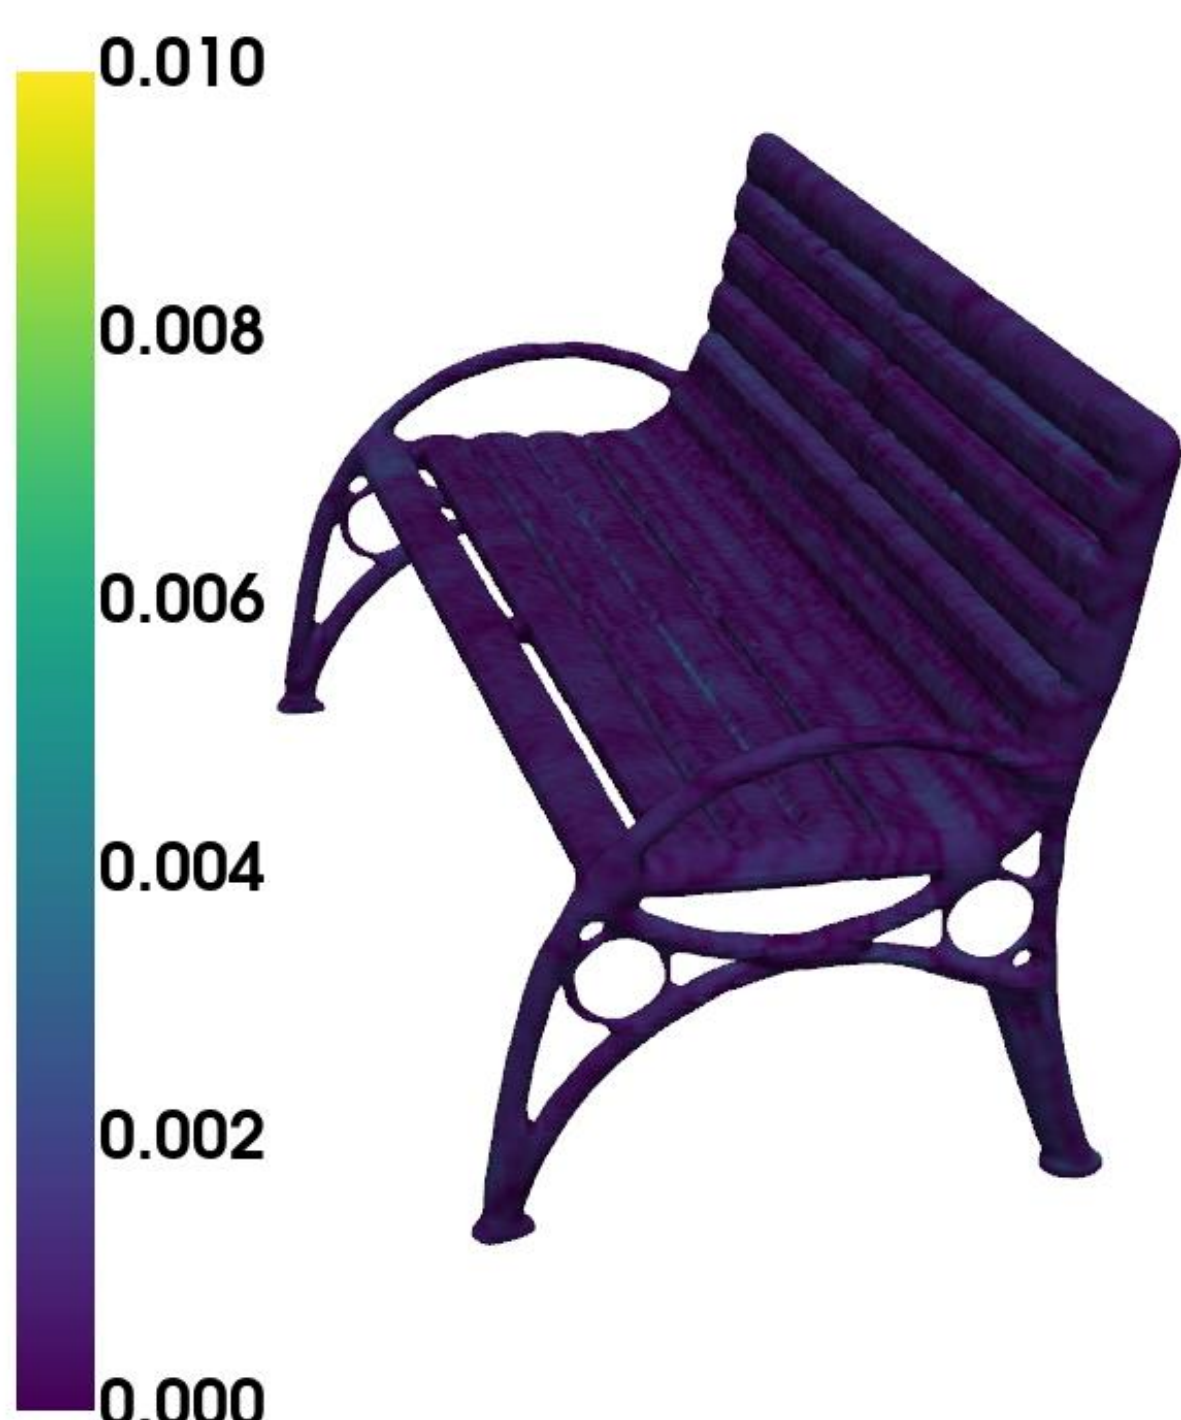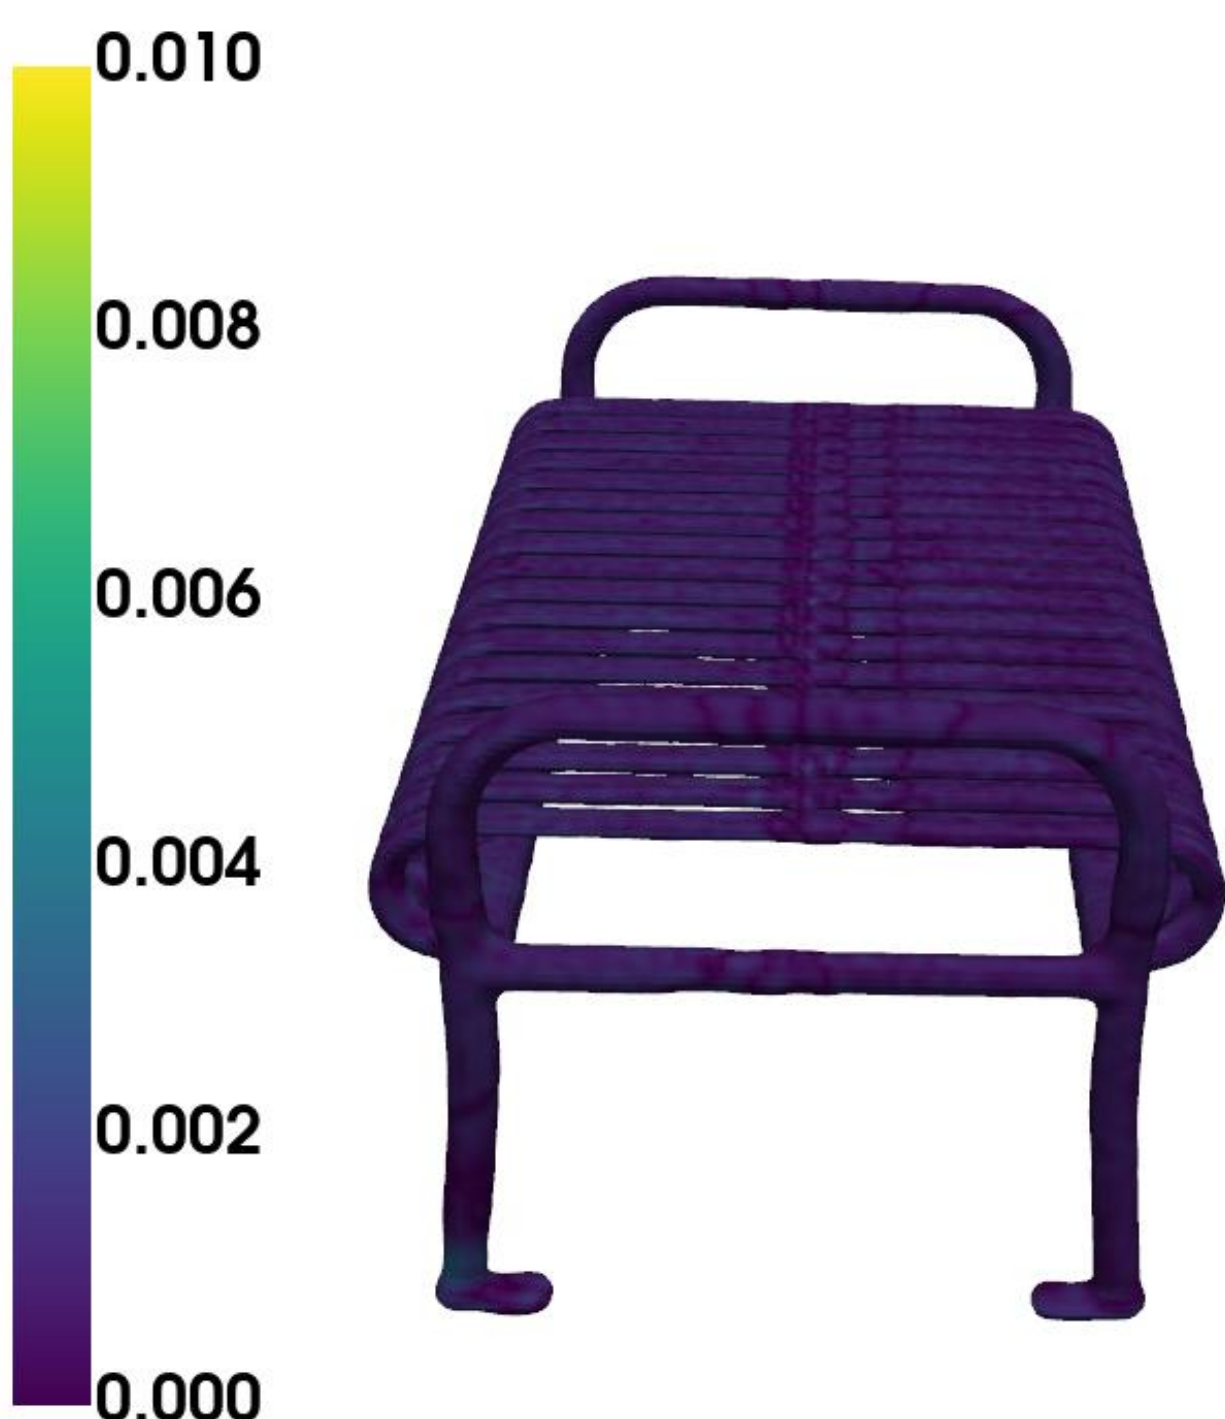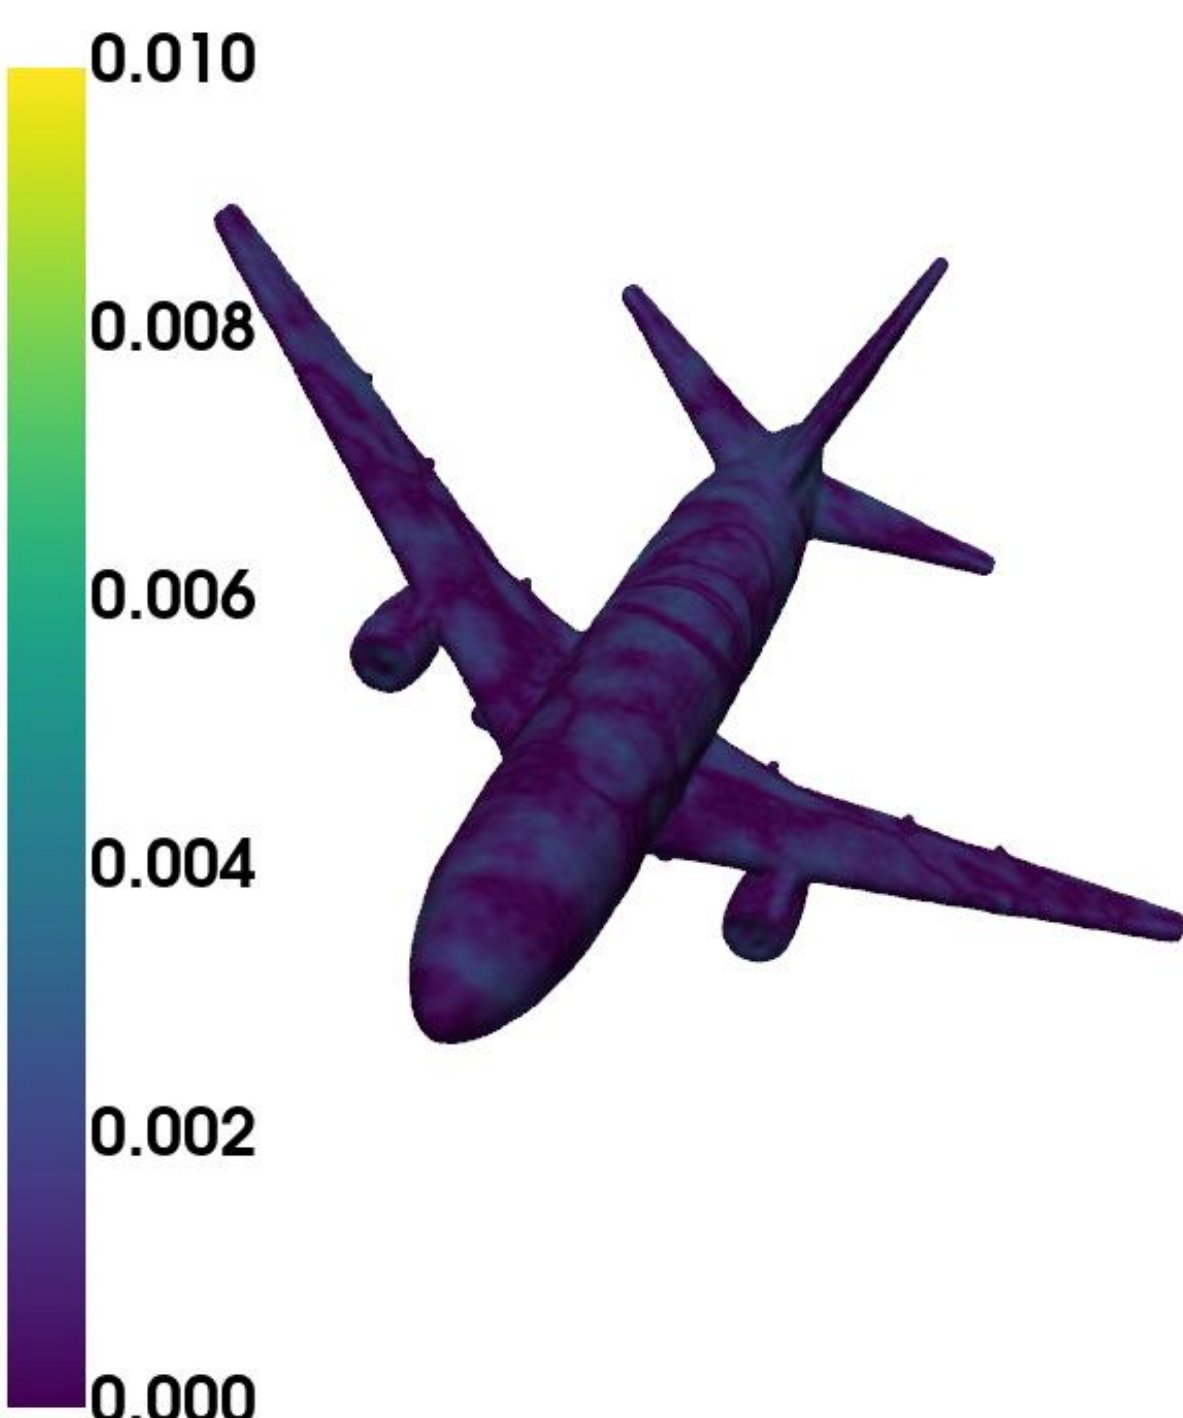



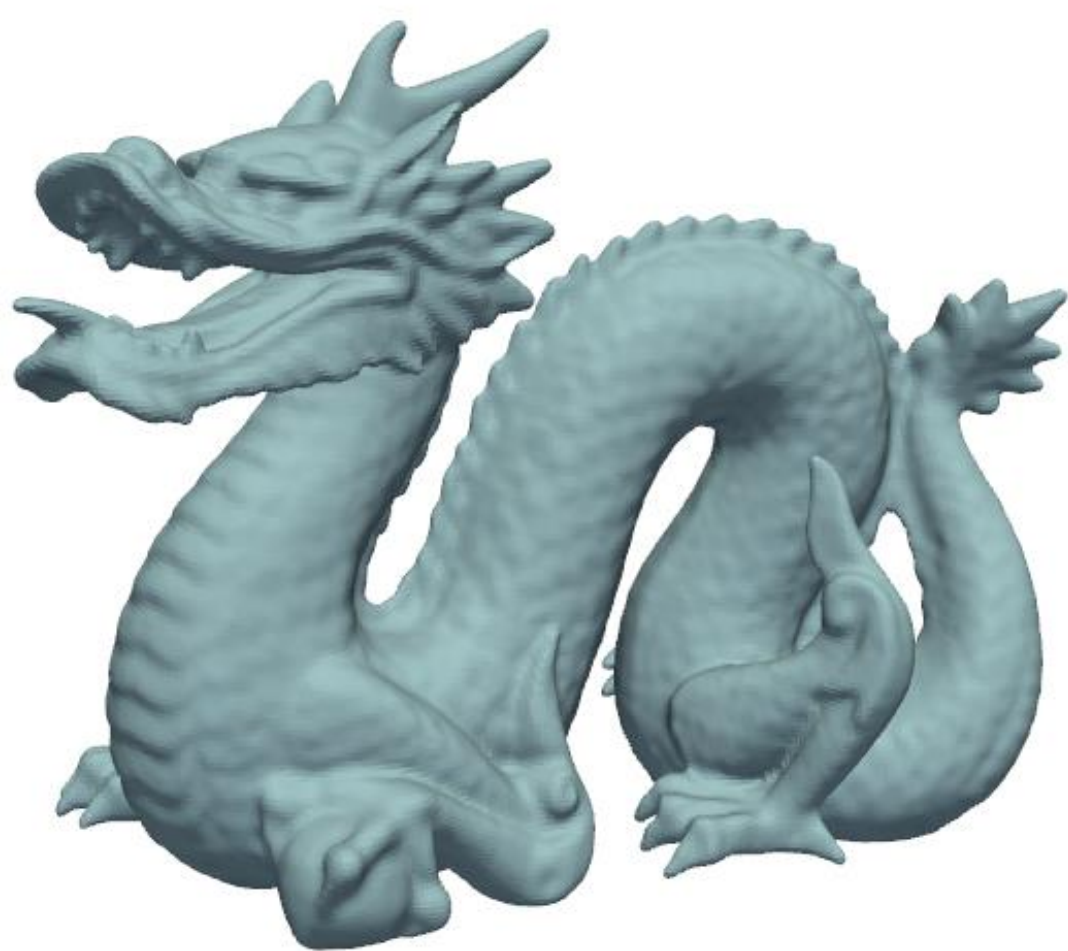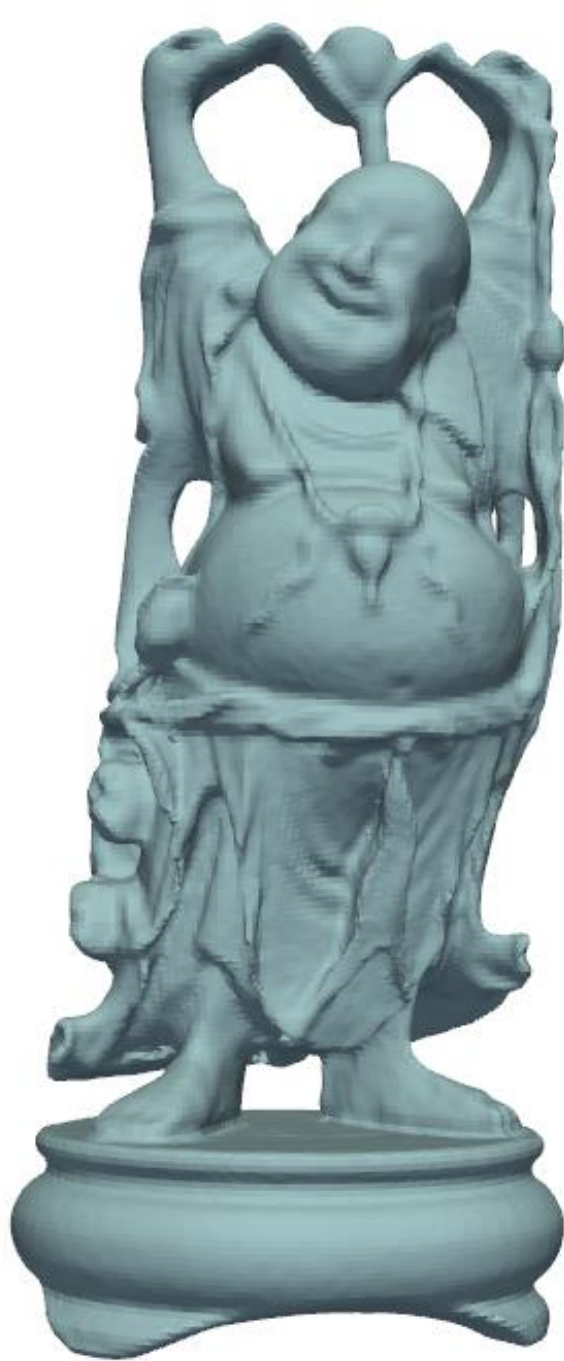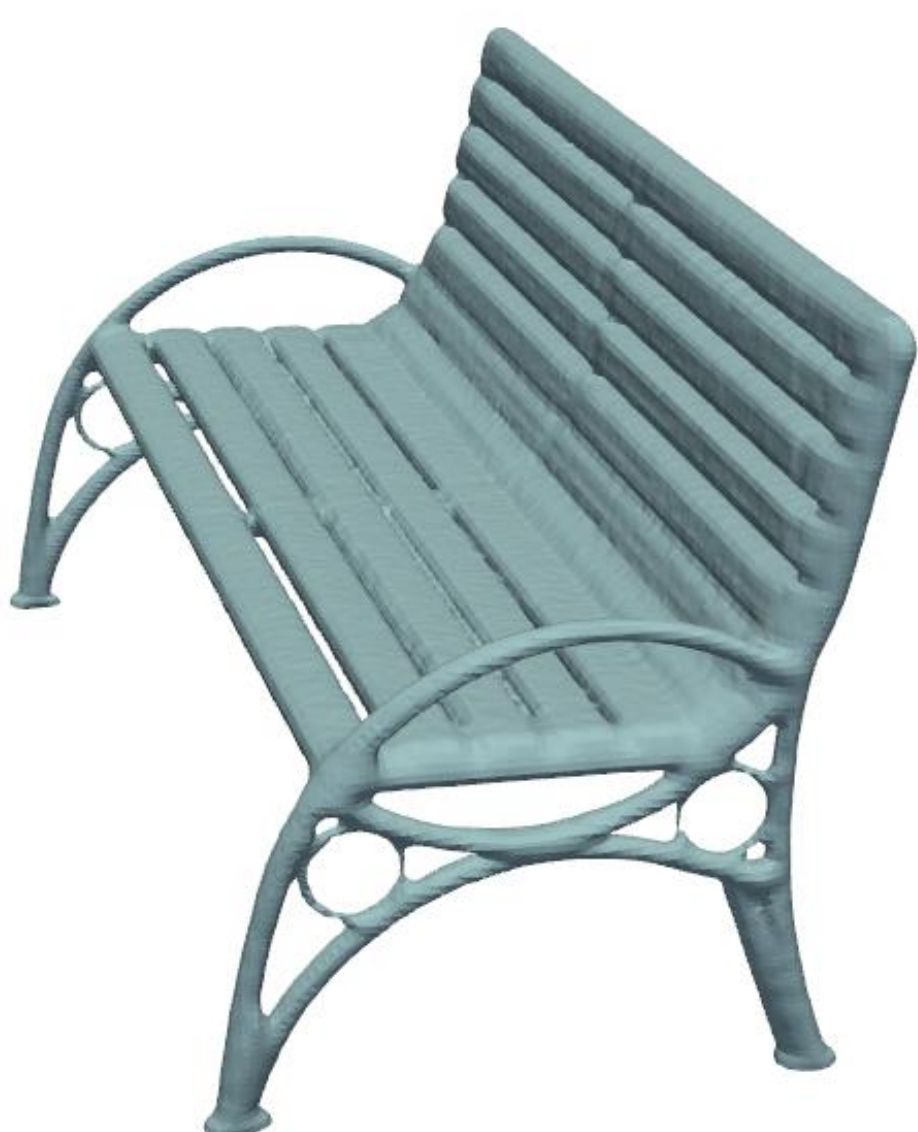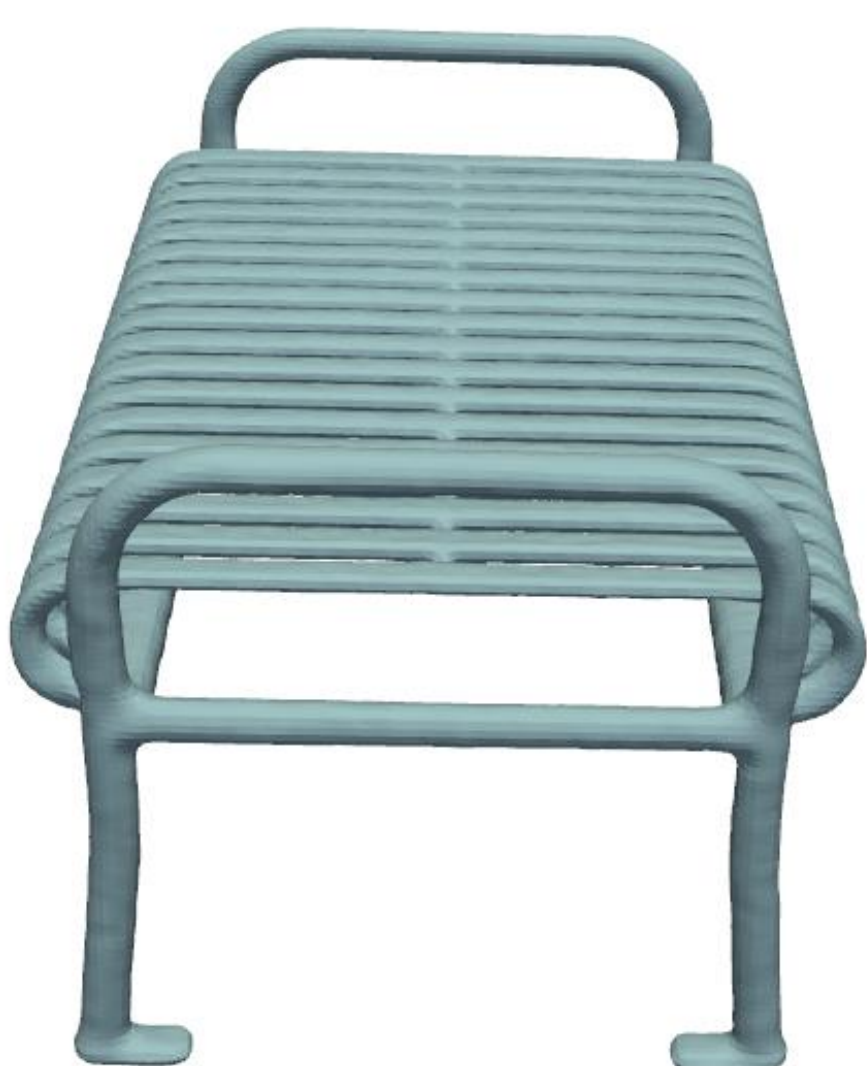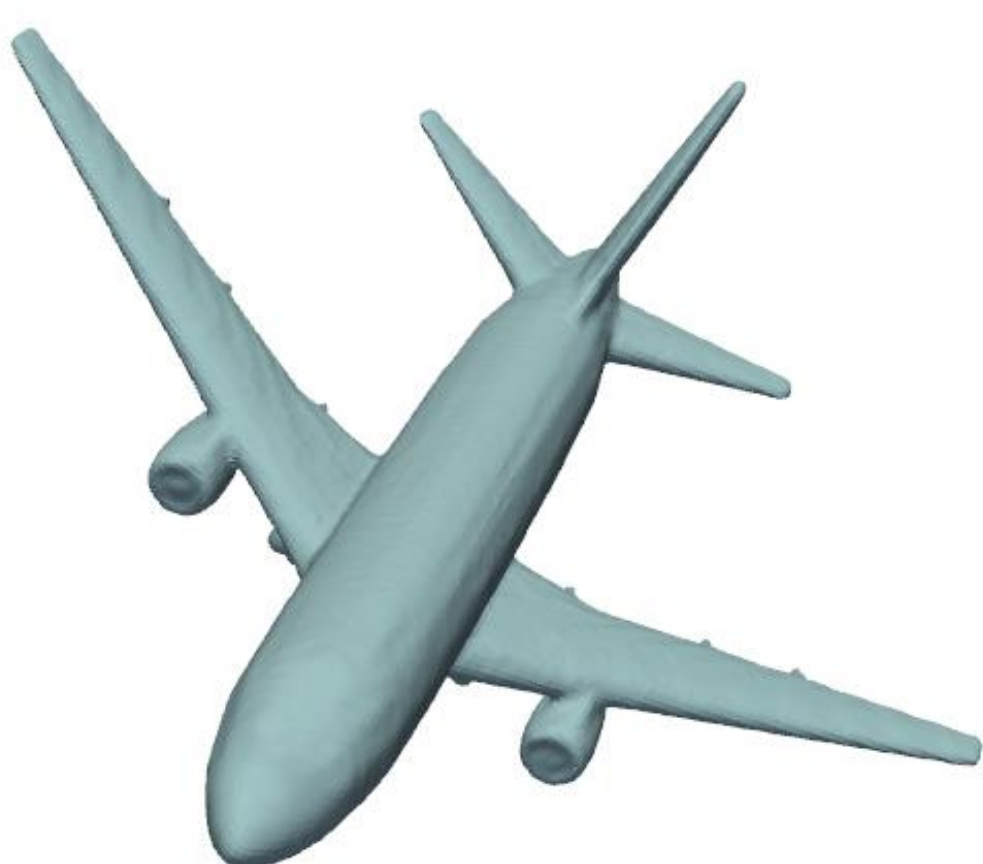



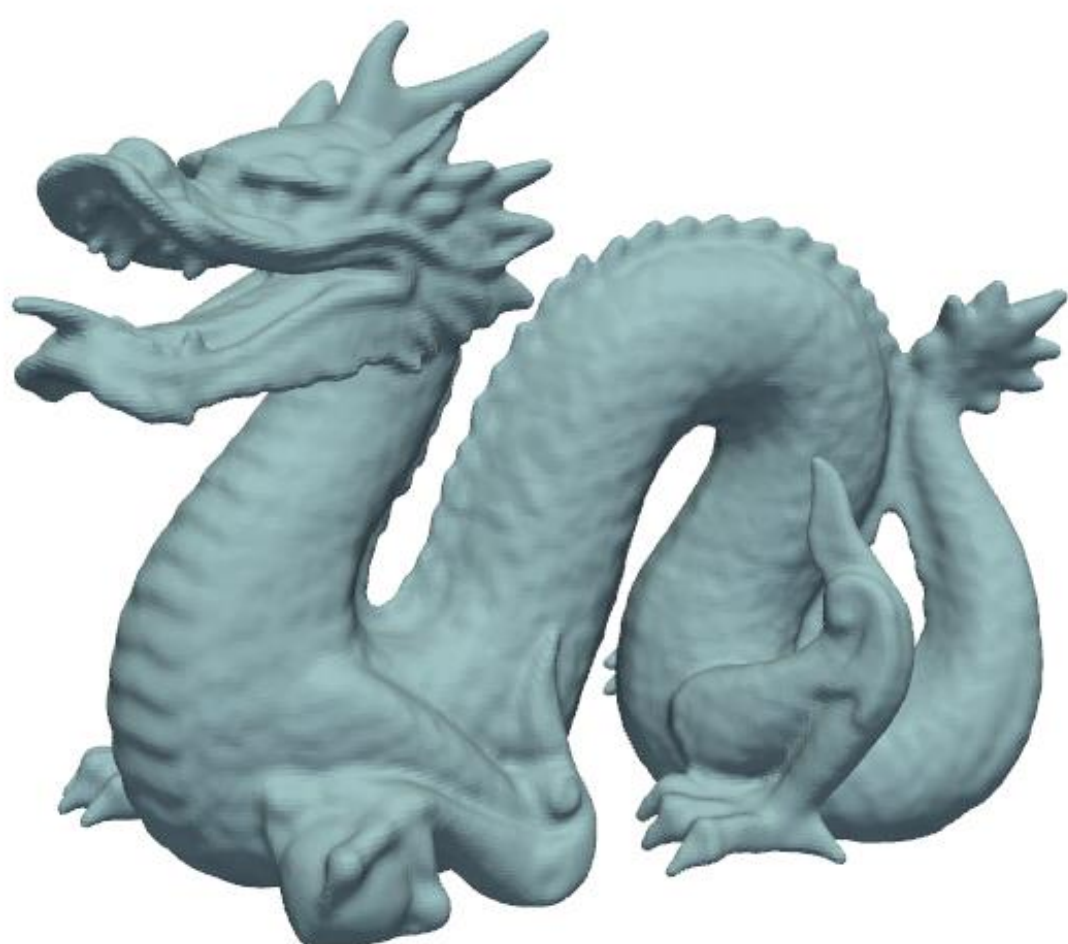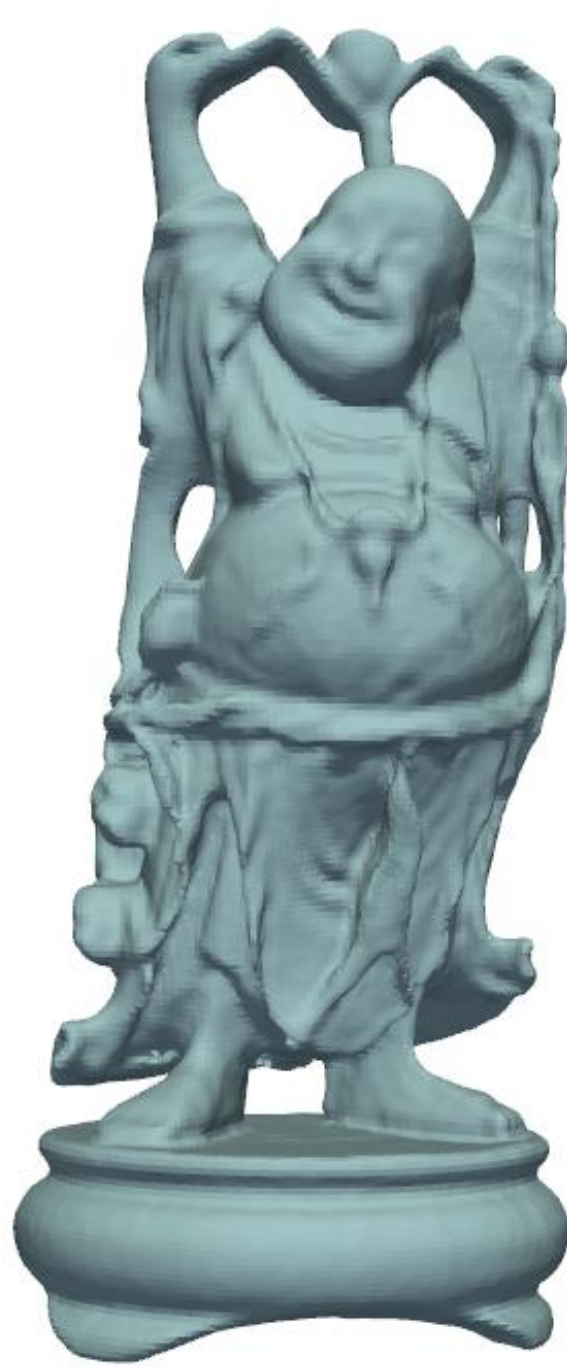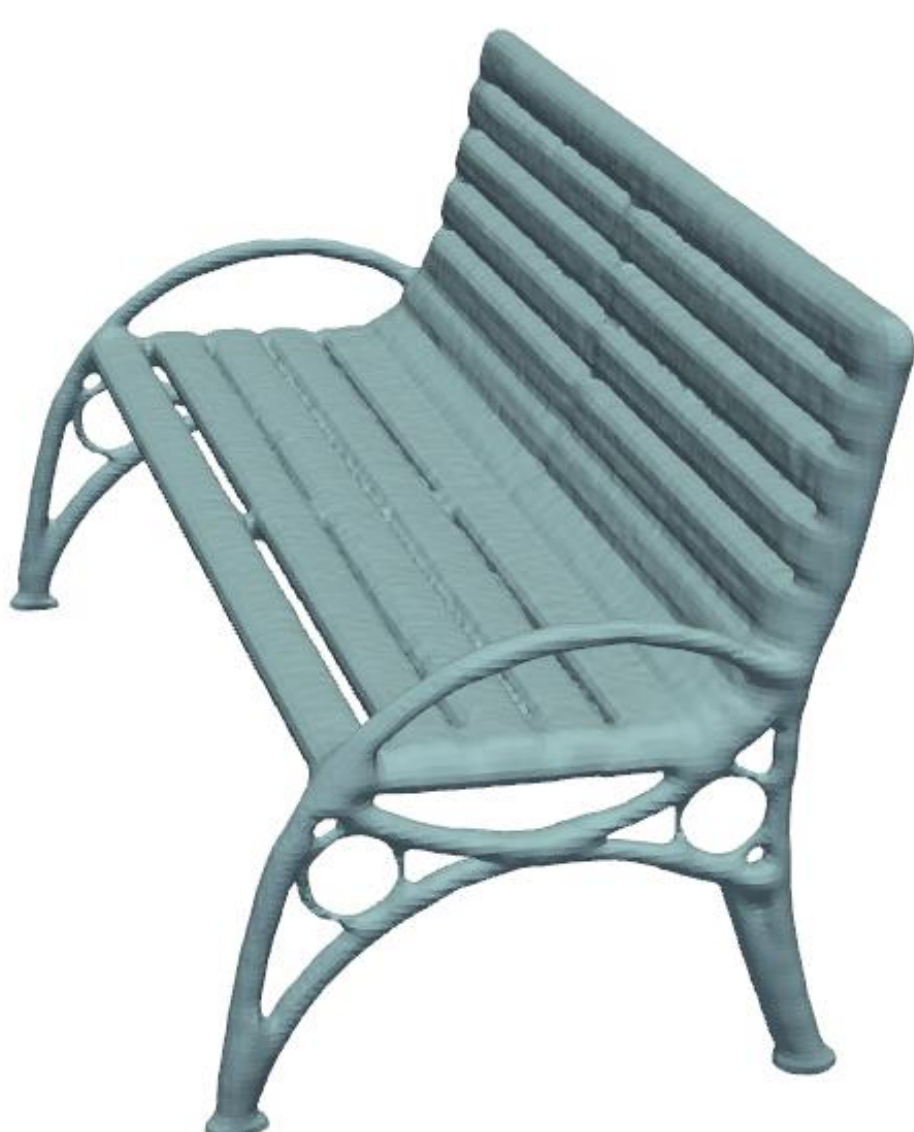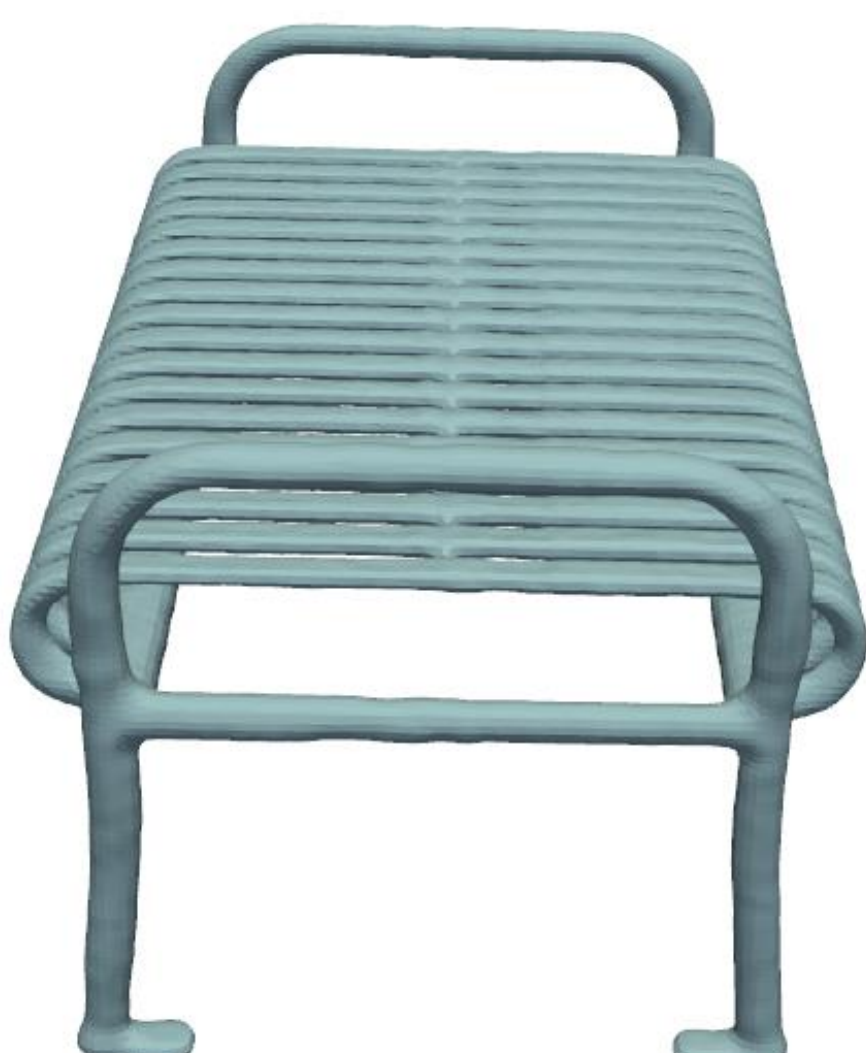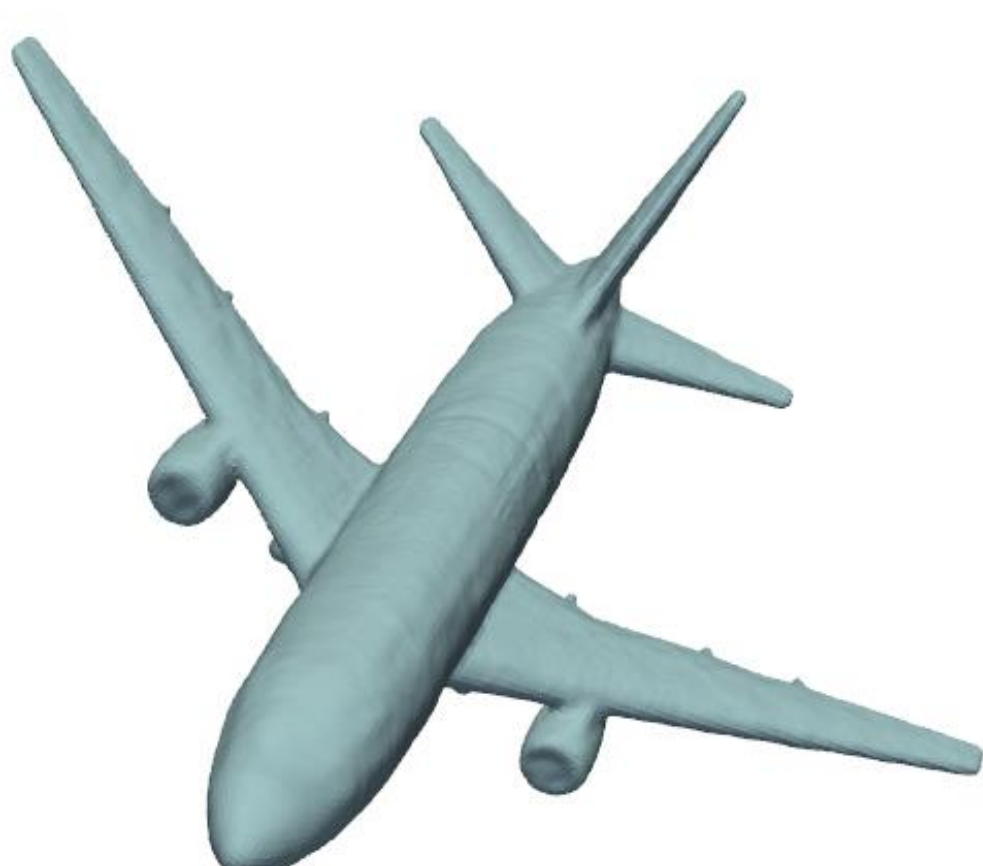



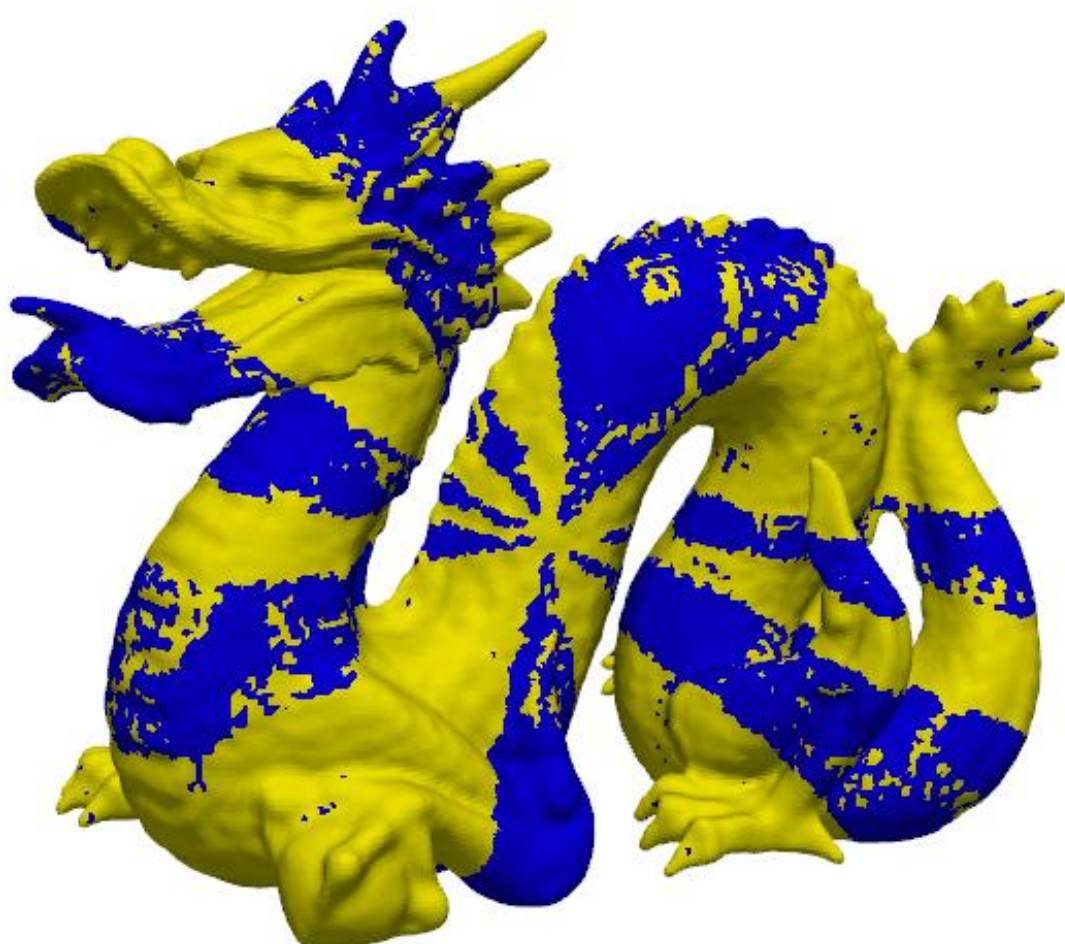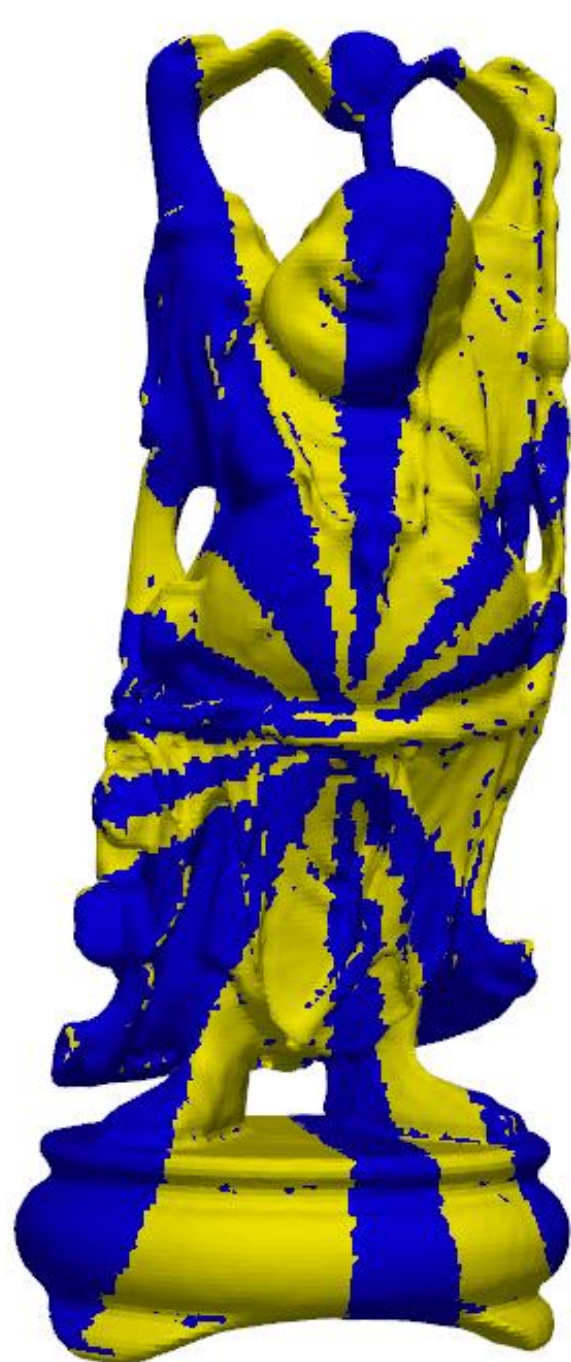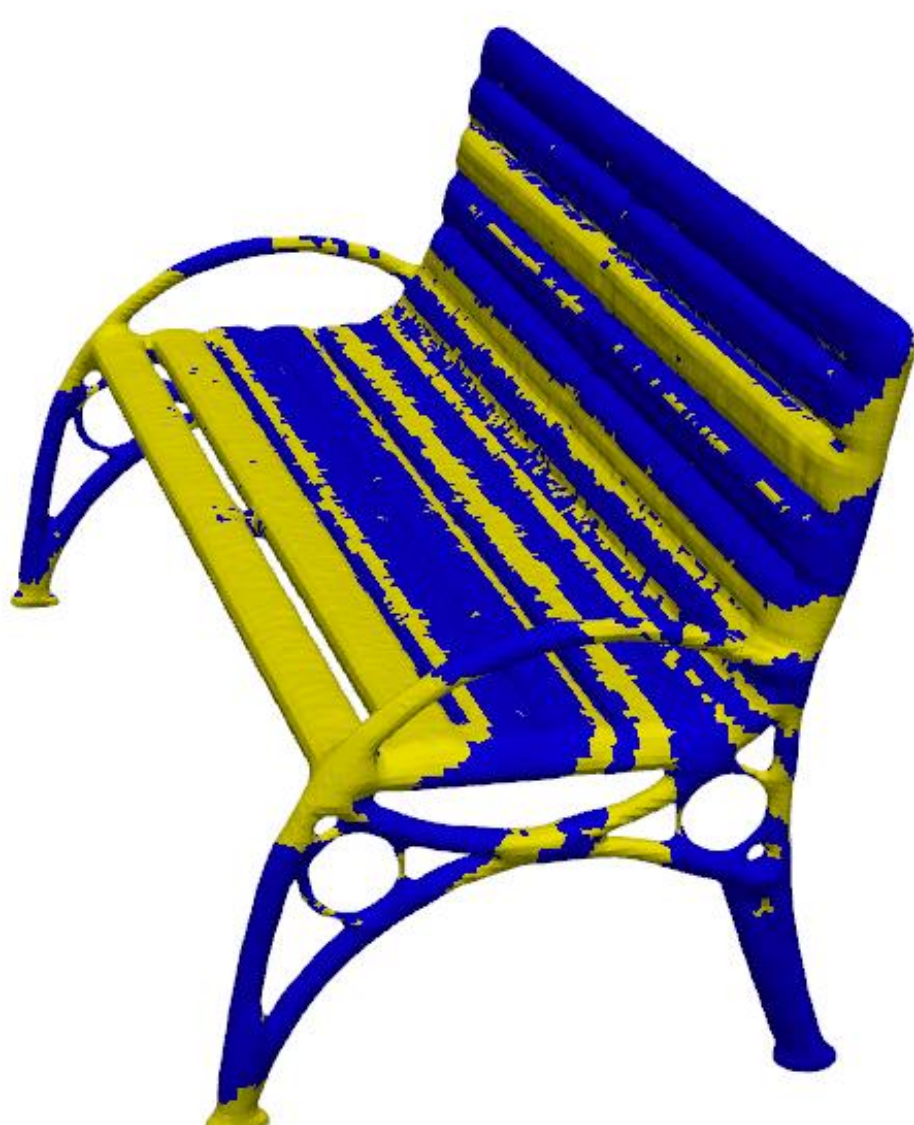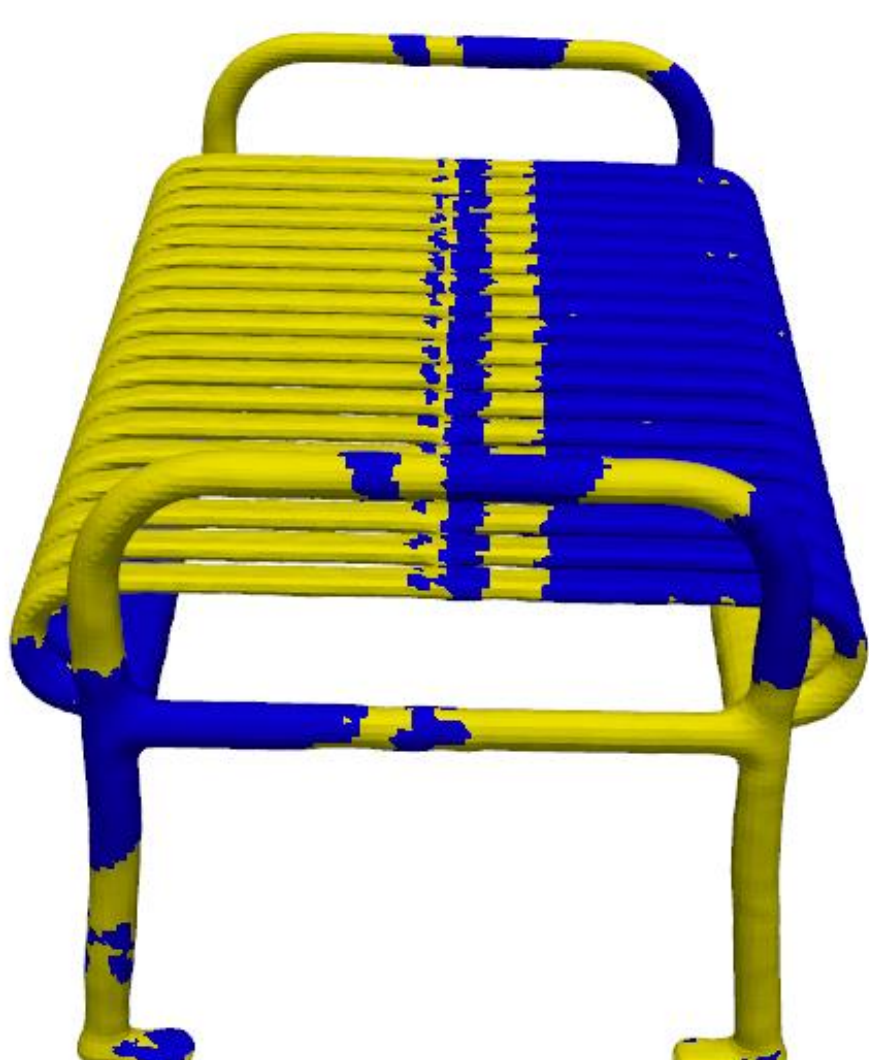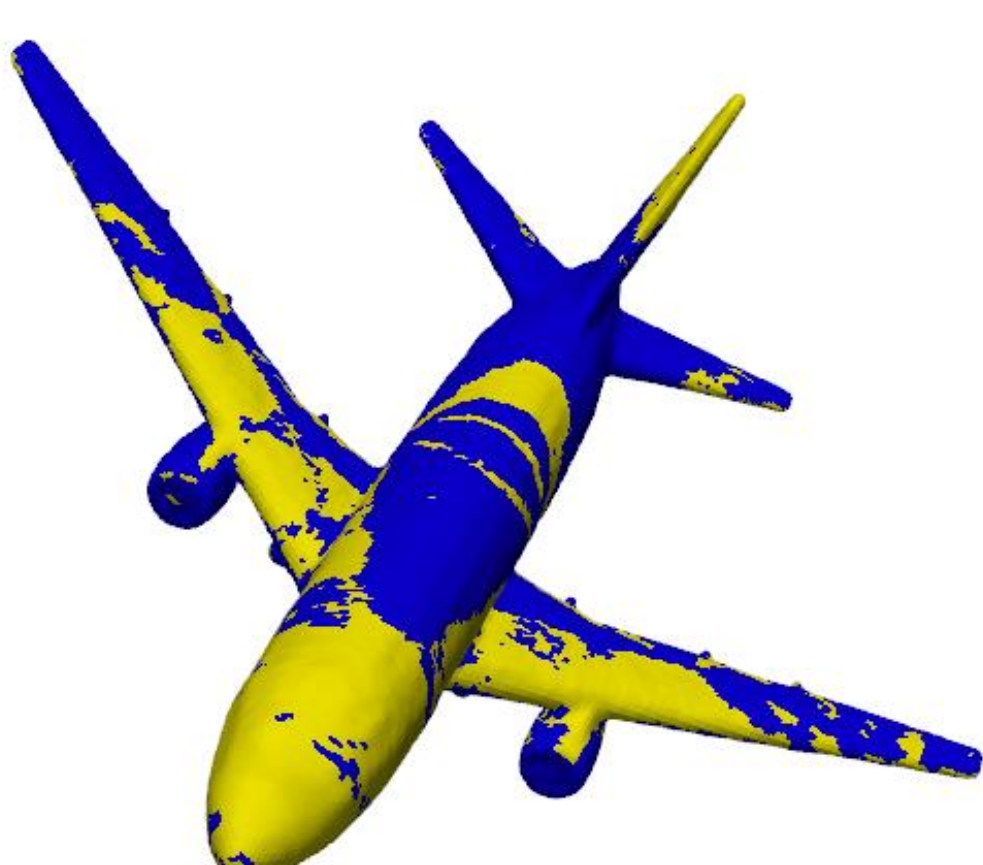

Supplement: Supplementary file 2 [file more_visual.pdf]
